# Supplementary material for: Accelerating Quantum Optimal Control of Multi-Qubit Systems with Symmetry-Based Hamiltonian Transformations
Source: arXiv:2309.05884 source file (2023-10-03)
Supplement: Supplementary file 1 [file Multi_Qubits_arXiv_SI.pdf]

# Supplementary Material for Accelerating Quantum Optimal Control of Multi-Qubit Systems with Symmetry-Based Hamiltonian Transformations[a]

Xian Wang,[1, b] Mahmut Sait Okay,[2] Anshuman Kumar,[2] and Bryan M. Wong[1, 2, 3, c]
[1] *Department of Physics & Astronomy, University of California-Riverside, 900 University Ave, Riverside, CA, 92521, United States*
[2] *Materials Science & Engineering Program, University of California-Riverside, 900 University Ave, Riverside, CA, 92521, United States*
[3] *Department of Chemistry, University of California-Riverside, 900 University Ave, Riverside, CA, 92521, United States*

## I. MATHEMATICAL METHODS

### A. Dynamics of Multi-Qubit Systems and Gradient-Based Quantum Optimal Control Algorithms

To provide the necessary background for the theoretical analyses used in our work, we first give a review of the mathematical methods in this section. We commence with a multi-qubit system built with spins. The state of entangled spins lies in the Hilbert space $\mathcal{H}(\mathbb{C}^{2^n})$ such that the dimension of the Hilbert space increases exponentially with $n$, the number of qubits. Other than establishing a foundation for quantum advantage, this exponential increase in the dimension of the Hilbert space poses significant challenges for simulating multi-qubit systems with classical computers.

The dynamics of a multi-qubit system are governed by the time-dependent Schrödinger equation

$$i\frac{\partial}{\partial t}|\psi(t)\rangle = (H_0 + H_c(t))\,|\psi(t)\rangle, \tag{1}$$

where $H_0$ is the static Hamiltonian, and $H_c(t)$ is the time-dependent control Hamiltonian. The static Hamiltonian,

$$H_0 = B_z \cdot \frac{1}{2}\sum_{i=1}^{n}\sigma_z^{(i)}, \tag{2}$$

can be realized by applying a uniform static magnetic field, $B_z$, that interacts with all the qubits along the $z$-axis. We denote $\sigma_z^{(i)}$ to be shorthand for the tensor product $\mathbb{I}_2^{\otimes i-1}\otimes\sigma_z\otimes\mathbb{I}_2^{\otimes n-i}$, where $\mathbb{I}_2$ is the rank-2 identity matrix. In many systems, such as the Ising model[1–3], each qubit is coupled to its neighbors. For a ring-shaped Ising model lattice, the static Hamiltonian becomes

$$H_0 = B_z \cdot \frac{1}{2}\sum_{i=1}^{n}\sigma_z^{(i)} + c_{\text{cpl}} \cdot \frac{1}{4}\sum_{i=1}^{n}\sigma_z^{(i)}\sigma_z^{(i+1)}, \tag{3}$$

where $c_{\text{cpl}}$ is the coupling coefficient that represents the strength at which each qubit is coupled to its nearest neighbor. Similarly, $\sigma_z^{(i)}\sigma_z^{(i+1)}$ is shorthand for the tensor product

---

[a] This article may be downloaded for personal use only. Any other use requires prior permission of the author and AIP Publishing. This article appeared in *AVS Quantum Science* and may be found at https://doi.org/10.1116/5.0162455.
[b] Electronic mail: xwang056@ucr.edu
[c] Electronic mail: bryan.wong@ucr.edu

$\mathbb{I}_2^{\otimes i-1} \otimes \sigma_z \otimes \sigma_z \otimes \mathbb{I}_2^{\otimes n-(i+1)}$, where the boundary condition $\sigma_z^{(n+i)} = \sigma_z^{(i)}, 1 \leq i \leq n$ holds. The control Hamiltonian

$$H_c = B_x(t) \cdot \frac{1}{2} \sum_{i=1}^{n} \sigma_x^{(i)} + B_y(t) \cdot \frac{1}{2} \sum_{i=1}^{n} \sigma_y^{(i)} \tag{4}$$

represents the scenario of simultaneously manipulating all of the qubits with time-dependent microwaves along the $x$- and $y$-axes. Transitions between quantum states can be realized by optimizing $B_x(t)$ and $B_y(t)$, the controlling pulses.

Given an initial state $|\psi(0)\rangle$, the final state $|\psi(T)\rangle$ can be formally calculated as follows:

$$|\psi(T)\rangle = \exp\left(-i \int_0^T (H_0 + H_c(t))\mathrm{d}t\right) |\psi(0)\rangle. \tag{5}$$

In contrast to conventional initial value problems in quantum dynamics, quantum optimal control (QOC) instead focuses on the inverse problem to construct optimal control pulses, $B_x(t)$ and $B_y(t)$, for evolving a multi-qubit system to a desired target state $|\psi_f\rangle$. To obtain numerical solutions to Eq. 5, we discretize the control duration $[0, T]$ into $N$ time steps of duration $\tau = \frac{T}{N}$. With this approximation, the propagator becomes

$$|\psi_{j+1}\rangle = \exp\left(-i\tau \left(H_0 + H_c[(j + \frac{1}{2})\tau]\right)\right) |\psi_j\rangle, \tag{6}$$

where $|\psi_j\rangle$ is the state at time step $t = j\tau$. We can evaluate the probability that the final state $|\psi_N\rangle$ transitions to the target state $|\psi_f\rangle$ with the following inner product:

$$P(|\psi_N\rangle) = |\langle\psi_f|\psi_N\rangle|^2. \tag{7}$$

As such, $P$ naturally forms a cost function for $B_x(t)$ and $B_y(t)$ that can be iteratively optimized with the gradient descent method as follows:

$$B_{j+\frac{1}{2}}^{(l+1)} = B_{j+\frac{1}{2}}^{(l)} + \gamma \frac{\mathrm{d}P}{\mathrm{d}B_{j+\frac{1}{2}}^{(l)}}, \tag{8}$$

where $B_{j+\frac{1}{2}}^{(l)}$ represents either $B_x$ or $B_y$ at $t = (j+\frac{1}{2})\tau$ in the $l$th iteration, and $\gamma$ is the update rate. The gradient $\frac{\mathrm{d}P}{\mathrm{d}B_{j+\frac{1}{2}}^{(l)}}$ can be evaluated using the chain rule[4,5]. The QOC numerical algorithm for constructing the optimized control field is given in Algorithm 1 below. Given the time interval, initial/target states, static Hamiltonian, and control Hamiltonian, the QOC algorithm outputs the final state and the optimized pulses that induce this transition.

All of the Hamiltonians mentioned above have some symmetry associated with a finite group. The Hamiltonians in Eqs. 2 and 4 have the symmetry of $S_n$, the permutation group, such that any permutation of the qubit indices does not change the Hamiltonians. The second term in Eq. 3 has the symmetry of $D_n$, the dihedral group, which is invariant under rotations and reflections of the qubits. Based on the symmetry of the multi-qubit system, the Hilbert space $\mathcal{H}(\mathbb{C}^{2^n})$ can be decomposed into orthogonal subspaces, and the Hamiltonians and propagators of the system can be transformed into a direct sum of blocks. In addition to accelerating the numerical calculations, this orthogonal decomposition of the Hilbert space brings natural symmetry-based protection to each of the subspaces and suppresses the room for quantum errors. In Secs. I B, I C, and I D, we introduce the methods for transforming the Hamiltonians based on their symmetry of finite groups.

### B. Transforming the Hamiltonians of $S_n$ Symmetry with the Young Method

The static Hamiltonian without coupling can be written explicitly as

$$H_0 = B_z \cdot \frac{1}{2} \sum_{i=1}^{n} \sigma_z^{(i)} = B_z \cdot \frac{1}{2}(\sigma_z \otimes \mathbb{I}_2^{\otimes n-1} + \mathbb{I}_2 \otimes \sigma_z \otimes \mathbb{I}_2^{\otimes n-2} + \cdots + \mathbb{I}_2^{\otimes n-1} \otimes \sigma_z). \tag{9}$$

**Algorithm 1:** QOC Algorithm

**Input:** time interval $[0, T]$, time step $\tau$, static Hamiltonian $H_0$, control Hamiltonian $H_c$, initial state $|\psi_0\rangle$, target state $|\psi_f\rangle$, initial guesses for $B_x^{(0)}(t), B_y^{(0)}(t)$
**Output:** final state $|\psi_N\rangle$, optimized $B_x(t), B_y(t)$

Define $H_0$, $H_c$, $|\psi_0\rangle$, $|\psi_f\rangle$
*thres* $\Leftarrow 0.999$, *maxIter* $\Leftarrow 100$
$l \Leftarrow 0$
Initialize $B_{j+1/2}^{(l)}$ **for** $j \Leftarrow 0, \ldots, N-1$
**while** $P <$ *thres* ***and*** $l <$ *maxIter* **do**
    **for** $j \Leftarrow 1, \ldots, N$ **do**
        Calculate $|\psi_j\rangle$ with Eq. 6
    **end**
    Update $P$ with Eq. 7
    **for** $j \Leftarrow N-1, \ldots, 0$ **do**
        Calculate $\frac{\mathrm{d}P}{\mathrm{d}B_{j+\frac{1}{2}}^{(l)}}$ using the chain rule
    **end**
    Calculate $\gamma$ with the golden-section search method
    Update $B_{j+1/2}^{(l+1)}$ **for** $j \Leftarrow 0, \ldots, N-1$ with Eq. 8
    $l \Leftarrow l + 1$
**end**
**return** $B_{j+1/2}$

The Hamiltonian in Eq. 9 obviously has $S_n$ symmetry since any permutation of the indices $i$ does not change the Hamiltonian but only rearranges the terms. Similarly, the control Hamiltonian in Eq. 4 also has $S_n$ symmetry. It should be noted that the group actions are exerted on the indices of the qubits, and if there are no coupling terms in the static Hamiltonian, the whole multi-qubit system has $S_n$ symmetry. $S_n$ symmetry, or some other finite group symmetry, originates from the fact that all of the qubits are homogeneous and distinguishable. In the context of this work, homogeneity indicates that all the qubits are described by the same Hamiltonians even though their indices are different. In our case, all the qubits are described with the same static ($B_z \cdot \frac{1}{2}\sigma_z$) and control ($B_x(t) \cdot \frac{1}{2}\sigma_x + B_y(t) \cdot \frac{1}{2}\sigma_y$) Hamiltonian.

We specify the tensor products of the eigenstates of $\sigma_z$ as the basis of the Hilbert space. Since both $\sigma_z$ and $\mathbb{I}_2$ are diagonal matrices, $H_z = \sum_{i=1}^{n} \sigma_z^{(i)}$ in Eq. 9 is diagonal; however, $H_x = \sum_{i=1}^{n} \sigma_x^{(i)}$ and $H_y = \sum_{i=1}^{n} \sigma_y^{(i)}$ are not. Using the commutation relation $[\sigma_j, \sigma_k] = 2i\varepsilon_{jkl}\sigma_l$, where $j, k, l = x, y, z$, it is obvious that $H_x$, $H_y$, and $H_z$ do not commute, and, thus, do not have eigenstates in common. Therefore, it is impossible to diagonalize $H_x$, $H_y$, and $H_z$ simultaneously. Nevertheless, the $S_n$ symmetry of the Hamiltonians leads to a second-best approach to construct a proper set of eigenstates of $H_z$. After being transformed with the unitary adjoint matrix made up of those eigenstates, $H_x$ and $H_y$ are block diagonalized while $H_z$ is left diagonal.

The first approach to obtain these eigenstates is to use the unitary irreducible representations (irreps) of $S_n$. We briefly introduce the Young method as follows.[6–8] Each irrep of $S_n$ can be characterized by a standard Young diagram made up of $n$ boxes. We denote the shape of the Young diagram as $\lambda$ and the corresponding irrep as $A^\lambda$. For qubit systems, we only consider the irreps characterized by Young diagrams made up of no more than two rows, i.e., $\lambda = [n-m, m], n-m \geq m, m \geq 0$. We then generate standard Young tableaux by filling each Young diagram with the numbers $1, 2, 3, \ldots, n$. The number of different standard Young tableaux $d_\lambda$ that can be generated for each Young diagram $\lambda$ is the dimension of the irrep $A^\lambda$. When $\lambda = [n-m, m]$ we have

$$d_\lambda = \frac{n!\,(n-2m+1)}{(n-m+1)!\,m!}. \tag{10}$$

We use the diagonal elements in each unitary irrep $A^\lambda$. For each group element $e_i \in S_n$, we denote its representation in $A^\lambda$ as $A^\lambda(e_i)$. We the following elements

$$O_j^\lambda = \sum_{i=1}^{n!} A_{jj}^\lambda(e_i)e_i,\ 1 \le j \le d_\lambda \tag{11}$$

in the group algebra $\mathcal{R}_{S_n}$ for each unitary irrep $A^\lambda$, where $A_{jj}^\lambda(e_i)$ is the $j$th diagonal element in the representation $A^\lambda(e_i)$. It should be noted that $A^\lambda$ in Eq. 11 must be unitary. For each standard Young tableau $T_j^\lambda$ with the shape $\lambda$, $1 \le j \le d_\lambda$, we define two permutation subgroups $R(T_j^\lambda)$, $C(T_j^\lambda)$ of $S_n$ as

$$\begin{aligned} R(T_j^\lambda) &= \{e \in S_n \mid e \text{ preserves the elements in each row of } T_j^\lambda\}, \\ C(T_j^\lambda) &= \{e \in S_n \mid e \text{ preserves the elements in each column of } T_j^\lambda\}. \end{aligned} \tag{12}$$

The Young symmetrizer of the tableau $T_j^\lambda$ can subsequently be defined as

$$Y(T_j^\lambda) = \sum_{e \in R(T_j^\lambda),\ e' \in C(T_j^\lambda)} \mathrm{sgn}(e')ee', \tag{13}$$

where $\mathrm{sgn}(e') : S_n \to \{1, -1\}$ is the sign of the permutation $e'$. With the Young symmetrizers, an irrep $A^\lambda$ can be derived, but it is not generally unitary and cannot be directly inserted into Eq. 11. The following recursive procedure yields the unitary irreps. Deleting the box filled with the largest remaining number repetitively for each Young tableau $T_j^\lambda$, we can define the standard Young tableau sequence $T_j^{\lambda,(0)} = T_j^\lambda, \ldots, T_j^{\lambda,(i)}, \ldots, T_j^{\lambda,(n-1)} = T^{[1]}$ where $\lambda, (i)$ is the shape of the Young diagram generated by deleting the boxes filled with the largest $i$ numbers in $T_j^\lambda$. Each Young tableau $T_j^{\lambda,(i)}$ corresponds to the group $S_{n-i}$ in the permutation group sequence $S_n \supset S_{n-1} \supset \cdots \supset S_1$. The recurrence relation is given as follows:

$$\begin{aligned} O_j^{\lambda,(n-1)} &= O^{[1]} = e_0, \\ O_j^{\lambda,(n-2)} &= \frac{d_{\lambda,(n-2)}}{2!} O^{[1]} Y(T_j^{\lambda,(n-2)}) O^{[1]}, \\ &\vdots \\ O_j^{\lambda,(i)} &= \frac{d_{\lambda,(i)}}{(n-i)!} O_j^{\lambda,(i+1)} Y(T_j^{\lambda,(i)}) O_j^{\lambda,(i+1)}, \\ &\vdots \\ O_j^{\lambda,(1)} &= \frac{d_{\lambda,(1)}}{(n-1)!} O_j^{\lambda,(2)} Y(T_j^{\lambda,(1)}) O_j^{\lambda,(2)}, \\ O_j^{\lambda,(0)} &= O_j^\lambda = \frac{d_\lambda}{n!} O_j^{\lambda,(1)} Y(T_j^\lambda) O_j^{\lambda,(1)}, \end{aligned} \tag{14}$$

where $e_0$ is the identity element in the group, and $d_{\lambda,(i)}$ is the dimension of the irrep $A^{\lambda,(i)}$ of $S_{n-i}$.

Using $|\uparrow\rangle$ and $|\downarrow\rangle$ to represent the spin-up and spin-down states of a single qubit, respectively, the index-permutation group action on the Fock basis

$$\alpha : S_n \times \{|\uparrow\rangle, |\downarrow\rangle\}^{\otimes n} \to \{|\uparrow\rangle, |\downarrow\rangle\}^{\otimes n} \tag{15}$$

can be defined as follows. Any element $e \in S_n$ can be defined with its action on the index sequence $[1, 2, \ldots, i, \ldots, n]$, i.e., $e \cdot [1, 2, \ldots, i, \ldots, n] \mapsto [p_1, p_2, \ldots, p_i, \ldots, p_n], p_i \in \{1, 2, \ldots, n\}$. Denoting any Fock state in $\{|\uparrow\rangle, |\downarrow\rangle\}^{\otimes n}$ as $|s_1, s_2, \ldots, s_i, \ldots, s_n\rangle, s_i = \uparrow, \downarrow$,

where $i$ is the index for the $i$th qubit, the index-permutation action is $e \cdot |s_1, s_2, \ldots, s_i, \ldots, s_n\rangle \mapsto |s_{p_1}, s_{p_2}, \ldots, s_{p_i}, \ldots, s_{p_n}\rangle$, e.g., $(1,2,3,4,5) \cdot |\uparrow\downarrow\uparrow\uparrow\downarrow\rangle \mapsto |\uparrow_2\downarrow_3\uparrow_4\uparrow_5\downarrow_1\rangle = |\downarrow\uparrow\downarrow\uparrow\uparrow\rangle$. In terms of the group algebra elements $O_j^\lambda = \sum_{i=1}^{n!} A_{jj}^\lambda(e_i)e_i, \lambda = [n-m, m], 1 \le j \le d_\lambda$, which is a linear combination of group elements, we define

$$O_j^\lambda \cdot |s_1, s_2, \ldots, s_i, \ldots, s_n\rangle = \sum_{i=1}^{n!} \left( A_{jj}^\lambda(e_i)(e_i \cdot |s_1, s_2, \ldots, s_i, \ldots, s_n\rangle) \right). \tag{16}$$

As such, $O_j^\lambda$ become operators acting on the Fock states, and it is trivial to show that for any number $m$, $0 \le m \le n$, the following set

$$\{|s_1, s_2, \ldots, s_i, \ldots, s_n\rangle \mid s_i = \uparrow, \downarrow; m \text{ of } \uparrow, (n-m) \text{ of } \downarrow\} \tag{17}$$

is an orbit in $\{|\uparrow\rangle, |\downarrow\rangle\}^{\otimes n}$ since any index-permutation action $e \in S_n$ does not convert a spin-up to a spin-down or inversely but only rearranges the spins.

Each operator $O_j^\lambda$ acts on no more than one element in each orbit. The elements to be acted on can be found with the Weyl tableaux that can be generated by filling the boxes in the Young diagram $\lambda = [n-m, m]$ with $\uparrow$ and $\downarrow$ entries. We next fill all the boxes in the second row with $\downarrow$ and all the boxes right above the second row with $\uparrow$ entries. The rest of the boxes (i.e., the boxes in the first row with no box below them) can be filled with either $\uparrow$ or $\downarrow$ so that no $\uparrow$ is to the right of any $\downarrow$. In this way, there are $n-2m+1$ different Weyl tableaux for each operator $O_j^\lambda$. It should be noted that the Young tableau $T_j^\lambda$ corresponding to $O_j^\lambda$ has the same shape with the Weyl tableaux, (i.e., $\lambda = [n-m, m]$). With the number $i$ in each box of the Young tableau $T_j^\lambda$ being the index for the spin in the same box of each Weyl tableau, $n-2m+1$ elements in $\{|\uparrow\rangle, |\downarrow\rangle\}^{\otimes n}$ will be generated. Obviously, each of them is an eigenstate of $H_z$ and belongs to a different orbit. Therefore, those $n-2m+1$ elements are orthogonal to each other. Acting $O_j^\lambda$ on the $n-2m+1$ elements, we obtain the orthogonal basis for a subspace of the Hilbert space $\mathcal{H}(\mathbb{C}^{2^n})$. Each basis vector is still an eigenstate of $H_z$. It can be shown that the subspaces generated by different $O_j^\lambda$ are orthogonal to each other, and we denote each subspace as $\mathcal{H}_j^\lambda$. The procedure above decomposes the Hilbert space $\mathcal{H}(\mathbb{C}^{2^n})$ with a dimension of $2^n$ into

$$\sum_{\lambda=[n-m,m]}^{n-m\ge m, m\ge 0} d_\lambda = \sum_{m=0}^{\lfloor n/2 \rfloor} \frac{n!\ (n-2m+1)}{(n-m+1)!\ m!} \tag{18}$$

orthogonal subspaces. Each subspace has a dimension of $n-2m+1$.

Thus far, with the Young method, we generated the orthogonal basis of the subspaces $\{\mathcal{H}_j^\lambda\}$. We next normalize the basis and let them be the columns of a unitary matrix $A_S$ such that the basis of each particular subspace is positioned together. Since all the columns of $A_S$ are eigenstates of $H_z$, after the unitary similarity transformation with the adjoint matrix $A_S$, $H_z' = A_S^\dagger H_z A_S$ remains diagonal. Moreover, after the same unitary similarity transformation, $H_x' = A_S^\dagger H_x A_S$ and $H_y' = A_S^\dagger H_y A_S$ are block diagonal. The nonzero elements in each block of $H_x'$ and $H_y'$ are distributed at the minor diagonals closest to the main diagonal (see Fig. 2 in the main text). The number of blocks equals the number of subspaces $\mathcal{H}_j^\lambda$ as described in Eq. 18, while the size of each block is consistent with the dimension of each subspace (i.e., $(n-2m+1) \times (n-2m+1)$).

Since the Hamiltonians in Eqs. 2 and 4 are block diagonal after the unitary similarity transformation with $A_S$, the evolution of a pure state $|\psi\rangle$ in any subspace $\mathcal{H}_j^\lambda$ is strictly confined within that subspace. In other words, if the initial state $|\psi(0)\rangle$ is in some subspace $\mathcal{H}_j^\lambda$, regardless of the temporal forms of the control pulses $B_x(t)$ and $B_y(t)$, the final state $|\psi(T)\rangle$ must also be in the same subspace. If the initial state is defined as a linear combination of states in multiple subspaces, i.e.,

$$|\psi(0)\rangle = \sum_{\lambda,j} c_j^\lambda |\psi_j^\lambda(0)\rangle, c_j^\lambda \in \mathbb{C}, |\psi_j^\lambda(0)\rangle \in \mathcal{H}_j^\lambda, \tag{19}$$

the final state must also be in those subspaces with the same probabilities, i.e.,

$$|\psi(T)\rangle = \sum_{\lambda,j} {c'}_j^{\lambda} |\psi_j^{\lambda}(T)\rangle, {c'}_j^{\lambda} \in \mathbb{C}, |\psi_j^{\lambda}(T)\rangle \in \mathcal{H}_j^{\lambda}, \|{c'}_j^{\lambda}\| = \|c_j^{\lambda}\|, \tag{20}$$

as long as the Hamiltonians preserve the $S_n$ symmetry. This implies that $\lambda$ is a good quantum number in a multi-qubit system with $S_n$ symmetry. Later we will show that $\lambda$ is equivalent to the quantum number $J$, the total spin angular momentum of the multi-qubit system. As such, we can then restrict the calculation of the Schrödinger equation (Eq. 1) within only necessary subspaces; i.e., instead of using the complete adjoint matrix $A_S$, we can define such an adjoint matrix $A'_S$ such that its columns consist of only the orthonormal basis of the subspaces in which the initial state $|\psi(0)\rangle$ lies. The transformed Hamiltonians $A'^{\dagger}_S H_x A'_S$, $A'^{\dagger}_S H_y A'_S$, and $A'^{\dagger}_S H_z A'_S$ will then have fewer blocks and a smaller size, while the calculation is not affected because the orthogonality of the subspaces guarantees that all omitted subspaces will not be transitioned into.

One disadvantage of the Young method is its computational complexity. Generating different $O_j^{\lambda}$ can take different runtimes, while the most time-consuming one, $O_1^{[n]}$, takes

$$O\left(\prod_{i=1}^{n} (i!)^{2^{n-i}}\right) \tag{21}$$

group operations to be generated. The table below summarizes the timing of the Young method for $3 \leq n \leq 7$. Obviously, it is not practical to generate the complete adjoint matrix $A_S$ with the Young method when $n$ is large. It should be noted that the orthogonal decomposition of the Hilbert space with the Young method,

$$\mathcal{H}(\mathbb{C}^{2^n}) = \bigoplus_{\lambda,j} \mathcal{H}_j^{\lambda}, \tag{22}$$

is used to generate the representation space of unitary groups, namely SU(2), in this study.[6–8] Therefore, the Clebsch-Gordan coefficients of SU(2), another method for generating the unitary irreps of SU(2), should lead to the same direct sum decomposition in Eq. 22, as we show in the next subsection.

Table S1: Comparison of computational runtimes for generating the adjoint matrix $A$ with different methods

| | Computational Walltime (seconds) | | |
|---|---|---|---|
| Number of qubits $n$ | Young method | CG coefficients of SU(2) | $D_n$ group algebra elements as operators |
| 3 | 0.0077 | 0.0024 | 0.0012 |
| 4 | 0.0178 | 0.0100 | 0.0023 |
| 5 | 0.4748 | 0.0428 | 0.0046 |
| 6 | 63.8318 | 0.1848 | 0.0356 |
| 7 | 21286.3550 | 0.8066 | 0.0245 |
| 8 | - | 3.4327 | 0.0581 |
| 9 | - | 14.5743 | 0.1380 |
| 10 | - | 61.0588 | 0.3467 |
| 11 | - | 258.1316 | 0.7800 |
| 12 | - | 1080.7927 | 1.8423 |
| 13 | - | 4436.7408 | 4.4299 |
| 14 | - | 18832.3390 | 11.1521 |

[a] Data collected with 8 Intel Broadwell CPUs. Computational timings for the Young method were not tested for 8 qubits and higher.

### C. Transforming the Hamiltonians of $S_n$ Symmetry with the Clebsch-Gordan Coefficients of SU(2)

The Clebsch-Gordan (CG) coefficients are the coefficients for the direct sum decomposition of the direct product of two group irreps. When there is no coupling between neighboring qubits, the $n$-qubit system can be described with $\mathrm{SU}(2)^{\otimes n}$, so we can focus on the CG coefficients of SU(2) in this section. The CG coefficients of SU(2), denoted as $\langle J_1, M_1; J_2, M_2 \mid J, M\rangle$, has an analytical expression. The angular momentum $J \in \{0, \frac{1}{2}, 1, \frac{3}{2}, 2, \dots\}$ and the angular momentum projection onto the $z$-axis $M \in \{-J, -J+1, \dots, J-1, J\}$ are good quantum numbers characterizing the orthonormal basis $|J, M\rangle$, i.e., $\langle J', M' \mid J, M\rangle = \delta_{J'J}\delta_{M'M}$. $\langle J_1, M_1; J_2, M_2 \mid J, M\rangle$ is nonzero if and only if $|J_1 - J_2| \leq J \leq J_1 + J_2$ and $M = M_1 + M_2$. When one of the two irreps is the 2-dimensional irrep (i.e., $J_2 = \frac{1}{2}$), the CG coefficients $\langle J_1, M_1; \frac{1}{2}, M_2 \mid J, M\rangle$ reduce to

$$\begin{aligned}
\left\langle J_1, M_1; \frac{1}{2}, \frac{1}{2} \;\middle|\; \left(J_1 + \frac{1}{2}\right), M \right\rangle &= \sqrt{\frac{J_1 + M + \frac{1}{2}}{2J_1 + 1}}, \\
\left\langle J_1, M_1; \frac{1}{2}, -\frac{1}{2} \;\middle|\; \left(J_1 + \frac{1}{2}\right), M \right\rangle &= \sqrt{\frac{J_1 - M + \frac{1}{2}}{2J_1 + 1}}, \\
\left\langle J_1, M_1; \frac{1}{2}, \frac{1}{2} \;\middle|\; \left(J_1 - \frac{1}{2}\right), M \right\rangle &= -\sqrt{\frac{J_1 - M + \frac{1}{2}}{2J_1 + 1}}, \\
\left\langle J_1, M_1; \frac{1}{2}, -\frac{1}{2} \;\middle|\; \left(J_1 - \frac{1}{2}\right), M \right\rangle &= \sqrt{\frac{J_1 + M + \frac{1}{2}}{2J_1 + 1}}.
\end{aligned} \tag{23}$$

The eigenstates of a single qubit can be written as $|\frac{1}{2}, \frac{1}{2}\rangle = |\uparrow\rangle$ and $|\frac{1}{2}, -\frac{1}{2}\rangle = |\downarrow\rangle$. When an additional qubit is added into the system, applying the CG coefficients in Eq. 23 gives the eigenstates of the two-qubit system, i.e., the symmetric triplet states $|1, 1\rangle = |\uparrow\uparrow\rangle$, $|1, 0\rangle = \frac{1}{\sqrt{2}}(|\uparrow\downarrow\rangle + |\downarrow\uparrow\rangle)$, $|1, -1\rangle = |\downarrow\downarrow\rangle$, and the anti-symmetric singlet state $|0, 0\rangle = \frac{1}{\sqrt{2}}(|\uparrow\downarrow\rangle - |\downarrow\uparrow\rangle)$. In other words, the procedure of the orthogonal decomposition of the Hilbert space $\mathcal{H}(\mathbb{C}^{2^n})$ of the combined two spin-$\frac{1}{2}$ systems is to decompose the direct product of two 2-dimensional irreps of SU(2) into the direct sum of two irreps. Similarly, when a new qubit is added to the multi-qubit system, the CG coefficients in Eq. 23 allow us to decompose the direct product of the irrep carried by each existing subspace and a 2-dimensional irrep into the direct sum of two if $J_1 > 0$, or one if $J_1 = 0$, irrep(s). In this way, the orthonormal basis of new orthogonal subspaces (i.e., the eigenstates of the multi-qubit system) can be generated.

Following the procedure above and iteratively applying Eq. 23, the eigenstates, $|J, M\rangle$, of a multi-qubit system with any number of qubits $n$ can be generated. These eigenstates are in different subspaces characterized by the angular momentum $J$, and we denote these subspaces as $\mathcal{H}^J$. Each $\mathcal{H}^J$ has a total of $2J+1$ basis kets $|J, M\rangle$. It is worth noting that different subspaces can have the same value of $J$. To distinguish among the subspaces $\{\mathcal{H}^J\}$ characterized by the same $J$, we require the evolution history of $J$. According to the CG coefficient $\langle J_1, M_1; \frac{1}{2}, M_2 \mid J, M\rangle$, the angular momentum $J$ of each subspace $\mathcal{H}^J$ of a $n$-qubit system and its counterpart $J_1$ of the $(n-1)$-qubit system satisfies the relation $J = J_1 + \frac{1}{2}$ or $J = J_1 - \frac{1}{2}$. We denote $J$ as $J^{(0)}$, $J_1$ as $J^{(1)}$, and the angular momentum in the $(n-2)$-qubit system as $J^{(2)}$. This sequence of angular momenta $J^{(0)} = J, J^{(1)}, J^{(2)}, \dots, J^{(n-1)} = \frac{1}{2}$ indicates how the subspace $\mathcal{H}^J$ is evolved to and is unique for each subspace. We can then use the evolution history of $J$, denoted as the sequence $J^{(n-1)}, \dots, J^{(i)}, \dots, J^{(0)}$, or $[J^{(i)}]$ for short, to distinguish each of the $\mathcal{H}^J$ with the same $J$. We denote each $\mathcal{H}^J$ with the evolution history $[J^{(i)}]$ as $\mathcal{H}^J_{[J^{(i)}]}$. Similar to the Young method in the previous subsection, we let the basis $|J, M\rangle$ in each $\mathcal{H}^J_{[J^{(i)}]}$ be the columns of the adjoint matrix $A_S$. After a unitary similarity transformation with $A_S$, $H'_z = A_S^\dagger H_z A_S$ remains diagonal, and $H'_x = A_S^\dagger H_x A_S$

and $H'_y = A_S^\dagger H_y A_S$ are block diagonal. Only the elements in the minor diagonals closest to the main diagonal in each block of $H'_x$ and $H'_y$ are nonzero. Therefore, $H_x$ and $H_y$ are the control Hamiltonians that change $M$ by $\pm 1$ but keep $J$ and $[J^{(i)}]$ unchanged. Further details are provided in Sec. I F.

Thus far, we have introduced two methods for transforming the Hamiltonians: utilizing the group algebra elements of $S_n$ with the Young method and decomposing the direct product of the irreps of SU(2) into a direct sum iteratively. Both methods decompose the Hilbert space $\mathcal{H}(\mathbb{C}^{2^n})$ into orthogonal subspaces $\{\mathcal{H}_j^\lambda\}$ or $\{\mathcal{H}_{[J^{(i)}]}^J\}$ and generate the orthonormal basis in each subspace. Since the two sets of subspaces both carry the irreps of SU(2), the basis of either set of subspaces can be linearly transformed to the other. In fact, denoting the adjoint matrix generated with the Young method as $A_S^{\mathrm{Y}}$ and that generated with the CG coefficients of SU(2) as $A_S^{\mathrm{CG}}$, tests for up to 7 qubits show that $A_S^{\mathrm{Y}\dagger} A_S^{\mathrm{CG}}$ is a permutation matrix (i.e., there is only one element of 1 in each row and column of $A_S^{\mathrm{Y}\dagger} A_S^{\mathrm{CG}}$, while the other elements are all 0, as shown in Fig. S1). Therefore, the adjoint matrices generated with the two methods are mathematically equivalent and only differ in the sorting of the subspaces.

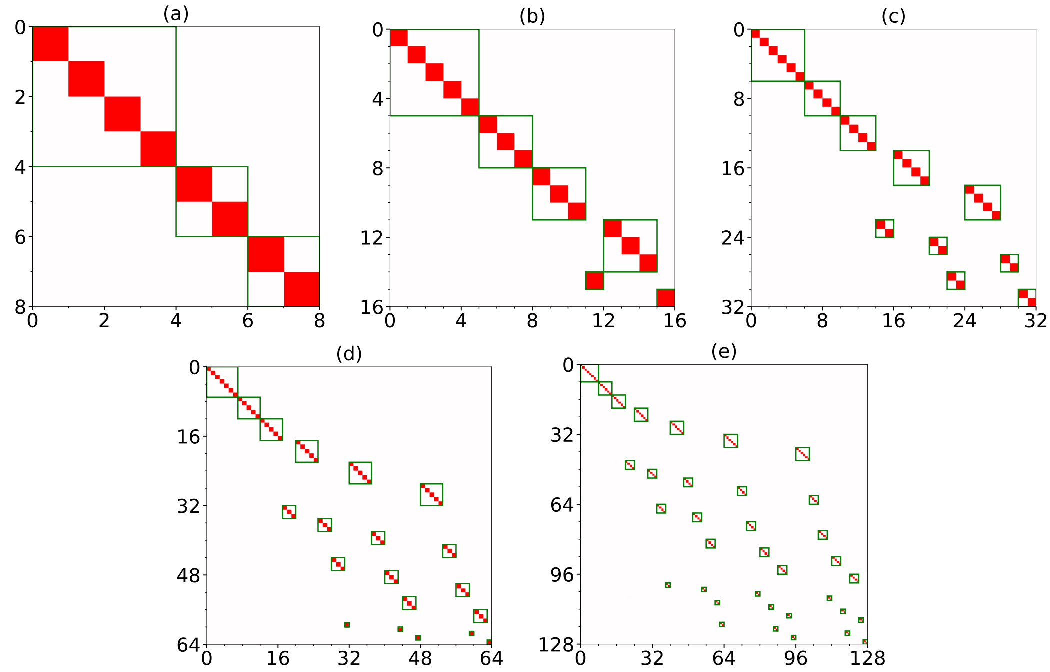


Figure S1: **Sparsity plots for $A_S^{\mathrm{Y}\dagger} A_S^{\mathrm{CG}}$ matrices of multi-qubit systems.** (a) 3-qubits; (b) 4-qubits; (c) 5-qubits; (d) 6-qubits; (e) 7-qubits. The $x$- and $y$-axes denote the column and row indices of the matrix elements, respectively. Each green-colored square box contains an identity matrix. All of the elements outside the boxes are zeros.

Since the orthonormal basis of the two sets of subspaces, $\{\mathcal{H}_j^\lambda\}$ and $\{\mathcal{H}_{[J^{(i)}]}^J\}$, are the same, the quantum numbers $\lambda = [n-m, m]$ and $J$ characterizing these subspaces must coincide with each other. It should be noted that the dimension of the subspace $\mathcal{H}_j^\lambda$ is $n - 2m + 1$ and that of $\mathcal{H}_{[J^{(i)}]}^J$ is $2J + 1$. The constraint $n - 2m + 1 = 2J + 1$ must be satisfied so that the subspaces $\mathcal{H}_j^\lambda$ and $\mathcal{H}_{[J^{(i)}]}^J$ can be the same. The index sets, $\{j\}$ and $\{[J^{(i)}]\}$, should also have the same number of elements so that there is a one-to-one mapping between them. Table S2 shows an example of the correspondence between $\{\mathcal{H}_j^\lambda\}$ and $\{\mathcal{H}_{[J^{(i)}]}^J\}$ of the 6-qubit system.

Table S2: Correspondence of good quantum numbers and indices between $\{\mathcal{H}_j^\lambda\}$ and $\{\mathcal{H}_{[J^{(i)}]}^J\}$ in a 6-qubit system

| Decomposition method | Young method | CG coefficients of SU(2) |
|---|---|---|
| Notation of subspace | $\mathcal{H}_j^\lambda$ | $\mathcal{H}_{[J^{(i)}]}^J$ |
| Good quantum number of subspaces | $\lambda = [n-m, m]$ | $J$ |
| Index of subspaces with the same good quantum number | $j$ | $[J^{(i)}] = [J^{(5)}, J^{(4)}, J^{(3)}, J^{(2)}, J^{(1)}, J^{(0)}]$ |
| Dimension of subspace | $n-2m+1$ | $2J+1$ |
| Good quantum number | $[6,0]$ | $3$ |
| Index of subspaces | 1, $[[1,2,3,4,5,6]]$ | $[\frac{1}{2}, 1, \frac{3}{2}, 2, \frac{5}{2}, 3]$ |
| Good quantum number | $[5,1]$ | $2$ |
| Index of subspaces | 1, $[[1,2,3,4,5],[6]]$ | $[\frac{1}{2}, 1, \frac{3}{2}, 2, \frac{5}{2}, 2]$ |
| | 2, $[[1,2,3,4,6],[5]]$ | $[\frac{1}{2}, 1, \frac{3}{2}, 2, \frac{3}{2}, 2]$ |
| | 3, $[[1,2,3,5,6],[4]]$ | $[\frac{1}{2}, 1, \frac{3}{2}, 1, \frac{3}{2}, 2]$ |
| | 4, $[[1,2,4,5,6],[3]]$ | $[\frac{1}{2}, 1, \frac{1}{2}, 1, \frac{3}{2}, 2]$ |
| | 5, $[[1,3,4,5,6],[2]]$ | $[\frac{1}{2}, 0, \frac{1}{2}, 1, \frac{3}{2}, 2]$ |
| Good quantum number | $[4,2]$ | $1$ |
| Index of subspaces | 1, $[[1,2,3,4],[5,6]]$ | $[\frac{1}{2}, 1, \frac{3}{2}, 2, \frac{3}{2}, 1]$ |
| | 2, $[[1,2,3,5],[4,6]]$ | $[\frac{1}{2}, 1, \frac{3}{2}, 1, \frac{3}{2}, 1]$ |
| | 3, $[[1,2,3,6],[4,5]]$ | $[\frac{1}{2}, 1, \frac{1}{2}, 1, \frac{1}{2}, 1]$ |
| | 4, $[[1,2,4,5],[3,6]]$ | $[\frac{1}{2}, 1, \frac{3}{2}, 1, \frac{1}{2}, 1]$ |
| | 5, $[[1,2,4,6],[3,5]]$ | $[\frac{1}{2}, 1, \frac{1}{2}, 0, \frac{1}{2}, 1]$ |
| | 6, $[[1,2,5,6],[3,4]]$ | $[\frac{1}{2}, 0, \frac{1}{2}, 1, \frac{1}{2}, 1]$ |
| | 7, $[[1,3,4,5],[2,6]]$ | $[\frac{1}{2}, 1, \frac{1}{2}, 1, \frac{3}{2}, 1]$ |
| | 8, $[[1,3,4,6],[2,5]]$ | $[\frac{1}{2}, 0, \frac{1}{2}, 1, \frac{3}{2}, 1]$ |
| | 9, $[[1,3,5,6],[2,4]]$ | $[\frac{1}{2}, 0, \frac{1}{2}, 0, \frac{1}{2}, 1]$ |
| Good quantum number | $[3,3]$ | $0$ |
| Index of subspaces | 1, $[[1,2,3],[4,5,6]]$ | $[\frac{1}{2}, 1, \frac{3}{2}, 1, \frac{1}{2}, 0]$ |
| | 2, $[[1,2,4],[3,5,6]]$ | $[\frac{1}{2}, 1, \frac{1}{2}, 1, \frac{1}{2}, 0]$ |
| | 3, $[[1,2,5],[3,4,6]]$ | $[\frac{1}{2}, 0, \frac{1}{2}, 1, \frac{1}{2}, 0]$ |
| | 4, $[[1,3,4],[2,5,6]]$ | $[\frac{1}{2}, 1, \frac{1}{2}, 0, \frac{1}{2}, 0]$ |
| | 5, $[[1,3,5],[2,4,6]]$ | $[\frac{1}{2}, 0, \frac{1}{2}, 0, \frac{1}{2}, 0]$ |

[a] The index of subspaces $j$ is not well-defined. We can rearrange the order of the diagonal elements in any representation of $S_n$ with a similarity transformation. Therefore, we pursue an index that is invariant under the similarity transformation of group representations. Note that the subspace $\mathcal{H}_j^\lambda$ is generated with the group algebra element $O_j^\lambda$ corresponding to a standard Young tableau $T_j^\lambda$ with the shape $\lambda$. Here we record the Young tableau $T_j^\lambda$ as a two-row list in addition to the index $j$, which is defined by sorting $T_j^\lambda$.

As shown in Table S2, we conclude that the Young method and the CG coefficients of SU(2) lead to the same decomposition of $\mathcal{H}(\mathbb{C}^{2^n})$, and the same transformation of the Hamiltonians $H_x$, $H_y$, $H_z$, whereas the CG coefficients method takes much less time, as shown in Table S1. In this work, we preferably use the CG coefficients of SU(2) to generate the adjoint matrix $A_S$ that transforms the Hamiltonians in Eqs. 2 and 4.

Although the Young method is cumbersome for transforming Hamiltonians with $S_n$ symmetry, it does imply that Hamiltonians with other types of finite group symmetries may be transformed in a similar way (i.e., to act the group algebra elements on some proper multi-qubit states). In the following subsection, we introduce how Hamiltonians with $D_n$ symmetry in Eq. 3 can be transformed with the group algebra elements of $\mathcal{R}_{D_n}$.

### D. Transforming the Hamiltonians of $D_n$ Symmetry

The dihedral group $D_n$ is the finite group describing the symmetry of a regular polygon with $n$ vertices. $D_n$ has $2n$ group elements, with $n$ rotational and $n$ reflective elements. The last term in Eq. 3 has $D_n$ symmetry since it is invariant under the rotations of the indices $\{i \in \mathbb{N} | 1 \leq i \leq n\}$, which are defined as

$$\begin{aligned} & i \mapsto (i+k) \bmod n && \text{if } (i+k) \bmod n \neq 0, \\ & i \mapsto n && \text{if } (i+k) \bmod n = 0, \\ & 1 \leq i \leq n, 0 \leq k \leq n-1, \end{aligned} \tag{24}$$

and the reflections of the indices, which are defined as

$$\begin{aligned} & i \mapsto (n+k-i) \bmod n && \text{if } (n+k-i) \bmod n \neq 0, \\ & i \mapsto n && \text{if } (n+k-i) \bmod n = 0, \\ & 1 \leq i \leq n, 0 \leq k \leq n-1. \end{aligned} \tag{25}$$

One intuitive way to understand $D_n$ symmetry is to position each qubit at the vertices of a $n$-gon and take the edges as the coupling between nearest neighbors. It should be noted that Eqs. 2 and 4 also have $D_n$ symmetry since $D_n$ is a subgroup of $S_n$. Therefore, the adjoint matrices block diagonalizing the coupling Hamiltonian, $H_{\text{cpl}} = \sum_{i=1}^{n} \sigma_z^{(i)} \sigma_z^{(i+1)}$, should block diagonalize $H_x$, $H_y$, and $H_z$ as well. We provide details on generating the adjoint matrices with the irreps of $D_n$ as follows.

The $2n$ elements of the $D_n$ group are in $\frac{n+3}{2}$ conjugate classes if $n$ is odd or $\frac{n}{2}+3$ conjugate classes if $n$ is even. Accordingly, the $D_n$ group has the same number of inequivalent irreps. The character tables of $D_n$ are given in Tables S3 and S4.

Table S3: Character table of the $D_n$ group for odd $n$

| | Conjugate class | | |
|---|---|---|---|
| Irrep | $\{e_0\}$ (1, 1) | $\{C_n^k, C_n^{n-k}\}$ (2, $\frac{n-1}{2}$) | $\{C_2^{(k)}\}$ ($n$, 1) |
| Identity (1) | 1 | 1 | 1 |
| $C_n$ (1) | 1 | 1 | -1 |
| $\theta_1 = \frac{2\pi}{n}$ (2) | 2 | 2cos($k\theta_1$) | 0 |
| $\vdots$ | $\vdots$ | $\vdots$ | $\vdots$ |
| $\theta_j = \frac{2\pi j}{n}$ (2) | 2 | 2cos($k\theta_j$) | 0 |
| $\vdots$ | $\vdots$ | $\vdots$ | $\vdots$ |
| $\theta_{\frac{n-1}{2}} = \frac{\pi(n-1)}{n}$ (2) | 2 | 2cos($k\theta_{\frac{n-1}{2}}$) | 0 |

[a] Three types of conjugate classes exist: (1) the identity element $\{e_0\}$, (2) rotations $\{C_n^k, C_n^{n-k}\}, 1 \leq k \leq \frac{n-1}{2}$, and (3) reflections $\{C_2^{(k)} | 0 \leq k \leq n-1\}$. The numbers in the bracket next to the conjugate classes are the number of elements in the class and the number of classes of that type. The irreps are 1- or 2-dimensional. Besides the identity irrep, the other 1-dimensional irrep is formed by the fact that the cyclic group $C_n$ is an invariant subgroup of $D_n$. The $\frac{n-1}{2}$ of 2-dimensional irreps are characterized by $\theta_j, 1 \leq j \leq \frac{n-1}{2}$. The number in the bracket next to the irreps is the dimension of the irrep.

The 2-dimensional irreps of $D_n$ can be constructed in the following way. In the $\theta_j = \frac{2\pi j}{n}$

Table S4: Character table of the $D_n$ group for even $n$

| Irrep | Conjugate class $\{e_0\}$ $(1,1)$ | $\{C_n^k, C_n^{n-k}\}$ $(2, \frac{n-2}{2})$ | $\{C_n^{\frac{n}{2}}\}$ $(1,1)$ | $\{C_2^{(k)}\}$ $(\frac{n}{2},1)$ | $\{C_2^{(k')}\}$ $(\frac{n}{2},1)$ |
|---|---|---|---|---|---|
| Identity (1) | 1 | 1 | 1 | 1 | 1 |
| $C_n$ (1) | 1 | 1 | 1 | -1 | -1 |
| $D_{\frac{n}{2}}$ (1) | 1 | 1 if $k$ is even<br>-1 if $k$ is odd | 1 if $\frac{n}{2}$ is even<br>-1 if $\frac{n}{2}$ is odd | -1 | 1 |
| $D'_{\frac{n}{2}}$ (1) | 1 | 1 if $k$ is even<br>-1 if $k$ is odd | 1 if $\frac{n}{2}$ is even<br>-1 if $\frac{n}{2}$ is odd | 1 | -1 |
| $\theta_1 = \frac{2\pi}{n}$ (2) | 2 | 2cos$(k\theta_1)$ | -2 | 0 | 0 |
| $\vdots$ | $\vdots$ | $\vdots$ | $\vdots$ | $\vdots$ | $\vdots$ |
| $\theta_j = \frac{2\pi j}{n}$ (2) | 2 | 2cos$(k\theta_j)$ | 2cos$(j\pi)$ | 0 | 0 |
| $\vdots$ | $\vdots$ | $\vdots$ | $\vdots$ | $\vdots$ | $\vdots$ |
| $\theta_{\frac{n-2}{2}} = \frac{\pi(n-2)}{n}$ (2) | 2 | 2cos$(k\theta_{\frac{n-2}{2}})$ | 2cos$(\frac{n-2}{2}\pi)$ | 0 | 0 |

[a] Five types of conjugate classes exist: (1) the identity element $\{e_0\}$, (2) rotations $\{C_n^k, C_n^{n-k}\}, 1 \leq k \leq \frac{n-2}{2}$, (3) rotation $\{C_n^{\frac{n}{2}}\}$, (4) reflections changing all the indices of the qubits $\{C_2^{(k)} | k = 2l, 0 \leq l \leq \frac{n}{2} - 1\}$, and (5) reflections keeping two indices of the qubits unchanged $\{C_2^{(k')} | k' = 2l+1, 0 \leq l \leq \frac{n}{2} - 1\}$. The numbers in the bracket next to the conjugate classes are the number of elements in the class and the number of classes of that type. The irreps are 1- or 2-dimensional. Besides the identity irrep, the other 1-dimensional irreps are formed by the fact that the cyclic group $C_n$ and $D_{\frac{n}{2}}$ are invariant subgroups of $D_n$. The $\frac{n-2}{2}$ of 2-dimensional irreps are characterized by $\theta_j, 1 \leq j \leq \frac{n-2}{2}$. The number in the bracket next to the irreps is the dimension of the irrep.

representation,

$$
\begin{aligned}
A(C_n^k) &= \begin{pmatrix} \cos(k\theta_j) & -\sin(k\theta_j) \\ \sin(k\theta_j) & \cos(k\theta_j) \end{pmatrix}, \\
A(C_2^{(k)}) &= \begin{pmatrix} \cos(k\theta_j) & \sin(k\theta_j) \\ \sin(k\theta_j) & -\cos(k\theta_j) \end{pmatrix}, \\
C_n^0 &= e_0, 0 \leq k \leq n-1.
\end{aligned} \tag{26}
$$

Here we clarify the definition of $C_n^k$ and $C_2^{(k)}$ with their action on the sequence of the indices of qubits $[1, 2, 3, \ldots, j, \ldots, n]$:

$$
\begin{aligned}
C_n^k \cdot [1, 2, 3, \ldots, n-1, n] &\mapsto [1+k, 2+k, \ldots, n-1, n, 1, 2, \ldots, k-1, k], \\
C_2^{(k)} \cdot [1, 2, 3, \ldots, n-1, n] &\mapsto [k, k-1, \ldots, 2, 1, n, n-1, \ldots, 2+k, 1+k], \\
C_2^{(k)} &= R \circ C_n^k, 0 \leq k \leq n-1,
\end{aligned} \tag{27}
$$

where $R$ is the action reversing the sequence and $\circ$ is the group operation. It is easy to verify that the matrices defined in Eq. 26 form the $\theta_j = \frac{2\pi j}{n}$ 2-dimensional representation and are compatible with the character tables in Tables S3 and S4.

Similar to the procedure in Sec. I B, we construct the elements

$$
O_j^\theta = \sum_{i=1}^{2n} A_{jj}^\theta(e_i) e_i, \ 1 \leq j \leq d_\theta \tag{28}
$$

in the group algebra $\mathcal{R}_{D_n}$ for each unitary irrep $A^\theta$. Here $\theta \in \{\text{Id}, C_n, \theta_1, \ldots, \theta_{\frac{n-1}{2}}\}$ (for odd $n$) or $\theta \in \{\text{Id}, C_n, D_{\frac{n}{2}}, D'_{\frac{n}{2}}, \theta_1, \ldots, \theta_{\frac{n-2}{2}}\}$ (for even $n$) is the index identifying the irrep,

and $A^{\theta}_{jj}(e_i)$ is the $j$th diagonal element in the representation $A^{\theta}(e_i)$ of the element $e_i \in D_n$, and $d_\theta = 1$ or 2 is the dimension of the representation $A^\theta$. It is trivial to show there are $n+1$ elements if $n$ is odd, or $n+2$ elements if $n$ is even, in the group algebra $\mathcal{R}_{D_n}$. These elements can be regarded as operators acting on the Fock basis. With the group actions defined in the mapping in Eq. 27, the action of any $e \in D_n$ on any Fock state $|s_1, s_2, s_3, \ldots, s_i, \ldots, s_n\rangle \in \{|\uparrow\rangle, |\downarrow\rangle\}^{\otimes n}$ can be defined as

$$\begin{aligned} C_n^k \cdot |s_1, s_2, s_3, \ldots, s_{n-1}, s_n\rangle &\mapsto |s_{1+k}, s_{2+k}, \ldots, s_{n-1}, s_n, s_1, s_2, \ldots, s_{k-1}, s_k\rangle, \\ C_2^{(k)} \cdot |s_1, s_2, s_3, \ldots, s_{n-1}, s_n\rangle &\mapsto |s_k, s_{k-1}, \ldots, s_2, s_1, s_n, s_{n-1}, \ldots, s_{2+k}, s_{1+k}\rangle, \\ 0 \le k \le n-1, s_i &\in \{|\uparrow\rangle, |\downarrow\rangle\}, 1 \le i \le n. \end{aligned} \tag{29}$$

The action of the operator $O^\theta_j = \sum_{i=1}^{2n} A^\theta_{jj}(e_i)e_i$ is the linear combination of the action of each $e_i \in D_n$, i.e.,

$$O^\theta_j \cdot |s_1, s_2, s_3, \ldots, s_i, \ldots, s_n\rangle = \sum_{i=1}^{2n} A^\theta_{jj}(e_i)(e_i \cdot |s_1, s_2, s_3, \ldots, s_i, \ldots, s_n\rangle). \tag{30}$$

With respect to the group action of $D_n$, $\{|\uparrow\rangle, |\downarrow\rangle\}^{\otimes n}$ is decomposed into orbits. Since $D_n$ has rotation and reflection elements only, it is not guaranteed that any two elements in the set $\{|s_1, s_2, s_3, \ldots, s_i, \ldots, s_n\rangle \mid s_i = \uparrow, \downarrow; m \text{ of } \uparrow, (n-m) \text{ of } \downarrow\}$ are equivalent to each other. Therefore, the set above is typically not an orbit of $\{|\uparrow\rangle, |\downarrow\rangle\}^{\otimes n}$ under the group action of $D_n$. However, it is trivial to show that the orbit $D_n \cdot |s_1, \ldots, s_n\rangle$ is a subset of the orbit $S_n \cdot |s_1, \ldots, s_n\rangle$ since any $D_n$ action also does not convert a spin-up to a spin-down or vice versa but only rearranges the spins. In other words, the fact that $D_n$ is a subgroup of $S_n$ results in the $D_n$ orbits being subsets of the $S_n$ orbits.

With the orbit-stabilizer theorem[9], we claim that for any $|s_1, \ldots, s_n\rangle \in \{|\uparrow\rangle, |\downarrow\rangle\}^{\otimes n}$, the number of elements in the orbit $D_n \cdot |s_1, \ldots, s_n\rangle$ is either a factor of $n$ if $C_n \cdot |s_1, \ldots, s_n\rangle = (D_n \backslash C_n) \cdot |s_1, \ldots, s_n\rangle$ or a factor of $2n$ if $C_n \cdot |s_1, \ldots, s_n\rangle \cap (D_n \backslash C_n) \cdot |s_1, \ldots, s_n\rangle = \varnothing$. Here, $D_n \backslash C_n = R \circ C_n$ is the difference of $D_n$ and $C_n$. The Hilbert space $\mathcal{H}(\mathbb{C}^{2^n})$ is decomposed into subspaces by acting each operator $O^\theta_j$ on some proper element(s) in the orbits. If $C_n \cdot |s_1, \ldots, s_n\rangle = (D_n \backslash C_n) \cdot |s_1, \ldots, s_n\rangle$, each operator $O^\theta_j$ acts on no more than one element in each orbit. In contrast, if $C_n \cdot |s_1, \ldots, s_n\rangle \cap (D_n \backslash C_n) \cdot |s_1, \ldots, s_n\rangle = \varnothing$, each operator $O^\theta_j$ acts on zero or two elements in each orbit. Following the procedure above, the orthogonal basis of all the subspaces is generated. Each subspace is defined by the group action of the operator $O^\theta_j$, and we denote that subspace as $\mathcal{H}^\theta_j$. We then normalize the orthogonal basis in each subspace $\mathcal{H}^\theta_j$ and let them be the columns of such a unitary matrix $A_D$ such that the basis of each particular subspace is positioned together. All the orthonormal basis vectors are the eigenstates of $H_{\text{cpl}}$ and $H_z$. Therefore, after the unitary similarity transformation with the adjoint matrix $A_D$, $H'_{\text{cpl}} = A^\dagger_D H_{\text{cpl}} A_D$ and $H'_z = A^\dagger_D H_z A_D$ remain diagonal, while $H'_x = A^\dagger_D H_x A_D$ and $H'_y = A^\dagger_D H_y A_D$ are block diagonal. It should be noted that the dimensions of the subspaces in the decomposition

$$\mathcal{H}(\mathbb{C}^{2^n}) = \bigoplus_{\theta, j} \mathcal{H}^\theta_j \tag{31}$$

are generally larger than those in the decomposition in Eq. 22. In fact, the dimension of $\mathcal{H}^{[n]}_1$ in the $S_n$ decomposition is $\sim O(n)$, whereas the dimension of $\mathcal{H}^{\text{Id}}_1$ in the $D_n$ decomposition is $\sim O(\frac{2^n}{n})$. Therefore, the sizes of the blocks in $H'_x$ and $H'_y$ after the $D_n$ transformation (which are equal to the dimensions of the subspaces) are generally larger than those corresponding to the $S_n$-induced transformation. Table S5 shows a comparison of the dimensions of $\mathcal{H}(\mathbb{C}^{2^n})$, $\mathcal{H}^{[n]}_1$, $\mathcal{H}^{\text{Id}}_1$ for $3 \le n \le 14$.

Similar to what we concluded in Sec. I B, with the Hamiltonians in Eqs. 3 and 4 block diagonalized with the $D_n$-induced unitary similarity transformation, it is clear that the

Table S5: Comparison of the dimensions of $\mathcal{H}(\mathbb{C}^{2^n})$, $\mathcal{H}_1^{[n]}$, and $\mathcal{H}_1^{\text{Id}}$

| | Dimension of space | | |
|---|---|---|---|
| Number of qubits $n$ | $\mathcal{H}(\mathbb{C}^{2^n})$ | $\mathcal{H}_1^{[n]}$ | $\mathcal{H}_1^{\text{Id}}$ |
| 3 | 8 | 4 | 4 |
| 4 | 16 | 5 | 6 |
| 5 | 32 | 6 | 8 |
| 6 | 64 | 7 | 13 |
| 7 | 128 | 8 | 18 |
| 8 | 256 | 9 | 30 |
| 9 | 512 | 10 | 46 |
| 10 | 1024 | 11 | 78 |
| 11 | 2048 | 12 | 126 |
| 12 | 4096 | 13 | 224 |
| 13 | 8192 | 14 | 380 |
| 14 | 16384 | 15 | 687 |

[a] The subspace $\mathcal{H}_1^{[n]}$ is generated with the operator $O_1^{[n]}$ of the identity representation of $S_n$, whereas the subspace $\mathcal{H}_1^{\text{Id}}$ is generated with the operator $O_1^{\text{Id}}$ of the identity representation of $D_n$. As such, they are listed together and compared to the complete Hilbert space $\mathcal{H}(\mathbb{C}^{2^n})$. The dimension of $\mathcal{H}(\mathbb{C}^{2^n})$, $\mathcal{H}_1^{[n]}$, and $\mathcal{H}_1^{\text{Id}}$ is $2^n$, $n+1$, and $\sim O(\frac{2^n}{n})$, respectively.

evolution of a pure state $|\psi\rangle$ in any subspace $\mathcal{H}_j^\theta$ is strictly confined within that subspace regardless of the temporal forms of the control pulses $B_x(t)$ and $B_y(t)$. Furthermore, if the initial state is defined as a linear combination of states in multiple subspaces, i.e.,

$$|\psi(0)\rangle = \sum_{\theta,j} c_j^\theta |\psi_j^\theta(0)\rangle, c_j^\theta \in \mathbb{C}, |\psi_j^\theta(0)\rangle \in \mathcal{H}_j^\theta, \tag{32}$$

the final state must also be in those subspaces with the same probabilities, i.e.,

$$|\psi(T)\rangle = \sum_{\theta,j} {c'}_j^\theta |\psi_j^\theta(T)\rangle, {c'}_j^\theta \in \mathbb{C}, |\psi_j^\theta(T)\rangle \in \mathcal{H}_j^\theta, \|{c'}_j^\theta\| = \|c_j^\theta\|. \tag{33}$$

This allows us to restrict the calculation of the Schrödinger equation in Eq. 1 within only necessary subspaces; i.e., instead of using the complete adjoint matrix $A_D$, we can define such an adjoint matrix $A'_D$ such that its columns consist of only the orthonormal basis of the subspaces in which the initial state $|\psi(0)\rangle$ lies. After the similarity transformation, the Hamiltonians in Eqs. 3 and 4 (i.e., $A'^\dagger_D H_0 A'_D$ and $A'^\dagger_D H_c A'_D$) will have a smaller size without affecting the calculation results.

Since the subspaces $\{\mathcal{H}_j^\theta\}$ are characterized by $\theta$, we conclude that $\theta$ is a good quantum number in a multi-qubit system with $D_n$ symmetry. It is worth noting that $\theta$ is no longer equivalent to the total spin angular momentum $J$; however, it can be shown that the angular momentum projection onto the $z$-axis $M$ is still a good quantum number for the eigenstates of $H_0$ in Eq. 3. For $S_n$ symmetry, where each $M \in \{-J, -J+1, \ldots, J-1, J\}$, there is only one eigenstate characterized with $M$ in each subspace $\mathcal{H}^J_{[J(i)]}$. In contrast, for $D_n$ symmetry, there may be more than one eigenstate characterized by the same $M$ in each subspace $\mathcal{H}_j^\theta$. It should be noted that $H_x$ and $H_y$ have $S_n$ symmetry and change $M$ by $\pm 1$. One consequence is that there may be nonzero elements not only in the minor diagonals closest to the main diagonal but also in further minor diagonals in the blocks of $H'_x = A_D^\dagger H_x A_D$ and $H'_y = A_D^\dagger H_y A_D$ (see Fig. 2 in the main text). We discuss the profile of $H'_x$ and $H'_y$ with the theory of creation/annihilation operators in Sec. I F.

### E. Mathematical Proof of the Orthogonality and Completeness of the Basis Vectors Generated by the $D_n$-Induced Decomposition of the Hilbert Space

In this subsection, we show that the basis vectors generated in the procedure in Sec. I D are orthogonal and complete in the Hilbert space $\mathcal{H}(\mathbb{C}^{2^n})$. For the proof, we construct the following complex 2-dimensional irreps of $D_n$. In the $\theta_j = \frac{2\pi j}{n}$ representation,

$$\begin{aligned} A(C_n^k) &= \begin{pmatrix} \exp(ik\theta_j) & 0 \\ 0 & \exp(-ik\theta_j) \end{pmatrix}, \\ A(C_2^{(k)}) &= \begin{pmatrix} 0 & \exp(ik\theta_j) \\ \exp(-ik\theta_j) & 0 \end{pmatrix}, \\ C_n^0 &= e_0, 0 \leq k \leq n-1, \end{aligned} \tag{34}$$

where $i$ is the imaginary unit. Similar to Eq. 27, we clarify the definition of $C_n^k$ and $C_2^{(k)}$ with their action on the sequence of the indices of qubits $[1, 2, 3, \ldots, j, \ldots, n]$:

$$\begin{aligned} C_n^k \cdot [1, 2, 3, \ldots, n-1, n] &\mapsto [1+k, 2+k, \ldots, n-1, n, 1, 2, \ldots, k-1, k]; \\ C_2^{(k)} \cdot [1, 2, 3, \ldots, n-1, n] &\mapsto [k, k-1, \ldots, 2, 1, n, n-1, \ldots, 2+k, 1+k], \\ C_2^{(k)} &= R \circ C_n^k, 0 \leq k \leq n-1, \end{aligned} \tag{35}$$

where $R$ is the action reversing the sequence and $\circ$ is the group operation. It is straightforward to verify that the matrices defined in Eq. 34 form the $\theta_j = \frac{2\pi j}{n}$, 2-dimensional representation and are compatible with the character tables in Tables S3 and S4. This complex irrep makes the proof simpler.

*Lemma 1.* For any $|s_1, \ldots, s_n\rangle \in \{|\uparrow\rangle, |\downarrow\rangle\}^{\otimes n}$, $C_n \cdot |s_1, \ldots, s_n\rangle$ and $(D_n \backslash C_n) \cdot |s_1, \ldots, s_n\rangle$ either are the same set or have no element in common.

*Proof.* Note that the reflection elements are defined by $C_2^{(k)} = R \circ C_n^k$. Then $R = R \circ e_0$ is also a reflection element. Considering that $C_n$ is an invariant subgroup of $D_n$, all the reflection elements form the coset $R \circ C_n = C_n \circ R = D_n \backslash C_n$.

If $R \cdot |s_1, \ldots, s_n\rangle \in C_n \cdot |s_1, \ldots, s_n\rangle$, we obviously have $(D_n \backslash C_n) \cdot |s_1, \ldots, s_n\rangle = (C_n \circ R) \cdot |s_1, \ldots, s_n\rangle = C_n \cdot (R \cdot |s_1, \ldots, s_n\rangle) = C_n \cdot |s_1, \ldots, s_n\rangle$.

Otherwise, if $R \cdot |s_1, \ldots, s_n\rangle \notin C_n \cdot |s_1, \ldots, s_n\rangle$, we have $(D_n \backslash C_n) \cdot |s_1, \ldots, s_n\rangle = (C_n \circ R) \cdot |s_1, \ldots, s_n\rangle = C_n \cdot (R \cdot |s_1, \ldots, s_n\rangle)$. Assume that some element $C_n^k \cdot (R \cdot |s_1, \ldots, s_n\rangle) \in C_n \cdot |s_1, \ldots, s_n\rangle$; then $(C_n^k)^{-1} \cdot (C_n^k \cdot (R \cdot |s_1, \ldots, s_n\rangle)) = ((C_n^k)^{-1} \circ C_n^k) \cdot (R \cdot |s_1, \ldots, s_n\rangle) = R \cdot |s_1, \ldots, s_n\rangle$ is in $(C_n^k)^{-1} \cdot (C_n \cdot |s_1, \ldots, s_n\rangle) = ((C_n^k)^{-1} \circ C_n) \cdot |s_1, \ldots, s_n\rangle = C_n \cdot |s_1, \ldots, s_n\rangle$, which is contradictory with $R \cdot |s_1, \ldots, s_n\rangle \notin C_n \cdot |s_1, \ldots, s_n\rangle$. We can then conclude that $(D_n \backslash C_n) \cdot |s_1, \ldots, s_n\rangle$ and $C_n \cdot |s_1, \ldots, s_n\rangle$ have no element in common if $R \cdot |s_1, \ldots, s_n\rangle \notin C_n \cdot |s_1, \ldots, s_n\rangle$.

*Lemma 2.* For any element $O_j^\theta = \sum_{i=1}^{2n} A_{jj}^\theta(e_i) e_i$ in the group algebra $\mathcal{R}_{D_n}$ as an operator on $|s_1, \ldots, s_n\rangle \in \{|\uparrow\rangle, |\downarrow\rangle\}^{\otimes n}$ as defined in Eq. 30, considering two different elements $|s_1', \ldots, s_n'\rangle$ and $|s_1'', \ldots, s_n''\rangle$ in $C_n \cdot |s_1, \ldots, s_n\rangle$, we have $O_j^\theta \cdot |s_1', \ldots, s_n'\rangle = c \times O_j^\theta \cdot |s_1'', \ldots, s_n''\rangle$, where $c \in \mathbb{C}$ is a complex coefficient that can be zero.

*Proof.* We discuss the operators $O_j^\theta$ by their corresponding irreps.

In the situation of the identity irrep, $O^{\text{Id}} = \sum_{i=1}^{2n} e_i$. Obviously, for any element $|s_1', \ldots, s_n'\rangle \in D_n \cdot |s_1, \ldots, s_n\rangle$, $O^{\text{Id}} \cdot |s_1', \ldots, s_n'\rangle$ is the same.

In the situation of the $C_n$ irrep, $O^{C_n} = \sum_{i=1}^{n} e_i - \sum_{i=n+1}^{2n} e_i$, where the elements in the first sum are rotations, and the elements in the second sum are reflections. Obviously, for any $|s_1', \ldots, s_n'\rangle \in C_n \cdot |s_1, \ldots, s_n\rangle$, $O^{C_n} \cdot |s_1', \ldots, s_n'\rangle$ is a zero vector if $C_n \cdot |s_1, \ldots, s_n\rangle = (D_n \backslash C_n) \cdot |s_1, \ldots, s_n\rangle$. Otherwise, for any $|s_1', \ldots, s_n'\rangle \in C_n \cdot |s_1, \ldots, s_n\rangle$, $O^{C_n} \cdot |s_1', \ldots, s_n'\rangle$ is the same if $C_n \cdot |s_1, \ldots, s_n\rangle \cap (D_n \backslash C_n) \cdot |s_1, \ldots, s_n\rangle = \varnothing$.

When $n$ is even, we need to discuss the two irreps formed by the fact that $D_{\frac{n}{2}}$ is an invariant subgroup of $D_n$. Following the notations in Table S4, we take these two operators as $O^{D_{\frac{n}{2}}} = \sum_{i=1}^{2n} A^{D_{\frac{n}{2}}}(e_i) e_i$ and $O^{D_{\frac{n}{2}}'} = \sum_{i=1}^{2n} A^{D_{\frac{n}{2}}'}(e_i) e_i$. Note that 1 and $-1$ appear

alternately as the coefficients of the $C_n$ elements and the $D_n\backslash C_n$ elements. Also, $C_n \cdot |s_1,\ldots,s_n\rangle$ and $(D_n\backslash C_n)\cdot|s_1,\ldots,s_n\rangle$ always have the same number of elements. Then for any $|s'_1,\ldots,s'_n\rangle \in C_n\cdot|s_1,\ldots,s_n\rangle$, $O^{D_{\frac{n}{2}}}\cdot|s'_1,\ldots,s'_n\rangle$ and $O^{D'_{\frac{n}{2}}}\cdot|s'_1,\ldots,s'_n\rangle$ must be zero vectors if $C_n\cdot|s_1,\ldots,s_n\rangle$ has an odd number of elements.

For $O^{D_{\frac{n}{2}}}\cdot|s'_1,\ldots,s'_n\rangle$ or $O^{D'_{\frac{n}{2}}}\cdot|s'_1,\ldots,s'_n\rangle$ to be a nonzero vector, we also need to ensure that the coefficients of the $C_n$ elements and those of the $D_n\backslash C_n$ elements, appearing as 1 and $-1$, do not cancel each other. If $C_n\cdot|s_1,\ldots,s_n\rangle \cap (D_n\backslash C_n)\cdot|s_1,\ldots,s_n\rangle = \varnothing$, it is obvious that those coefficients will not cancel each other since they are the coefficients of the elements in the two different sets $C_n\cdot|s_1,\ldots,s_n\rangle$ and $(D_n\backslash C_n)\cdot|s_1,\ldots,s_n\rangle$. Acting $O^{D_{\frac{n}{2}}}$ or $O^{D'_{\frac{n}{2}}}$ on other elements $|s''_1,\ldots,s''_n\rangle \in C_n\cdot|s_1,\ldots,s_n\rangle$ will result in a collinear basis vector with a global phase factor of 1 or $-1$.

We then discuss the situation of $C_n\cdot|s_1,\ldots,s_n\rangle = (D_n\backslash C_n)\cdot|s_1,\ldots,s_n\rangle$ where each has an even number of elements. In this case, there must be an element $C_n^k \in C_n$ such that $C_n^k\cdot|s'_1,\ldots,s'_n\rangle = R\cdot|s'_1,\ldots,s'_n\rangle$, where $R\in D_n\backslash C_n$ is the element reversing the sequence $|s'_1,\ldots,s'_n\rangle$. We notice that, following the notations in Table S4, the element $R$ is in the conjugate class $C_2^{(k)}$. For the case that the coefficient of $C_n^k$ is 1, $O^{D_{\frac{n}{2}}}\cdot|s'_1,\ldots,s'_n\rangle$ is a zero vector, and $O^{D'_{\frac{n}{2}}}\cdot|s'_1,\ldots,s'_n\rangle$ is a nonzero vector. Otherwise, if the coefficient of $C_n^k$ is $-1$, $O^{D_{\frac{n}{2}}}\cdot|s'_1,\ldots,s'_n\rangle$ is a nonzero vector, and $O^{D'_{\frac{n}{2}}}\cdot|s'_1,\ldots,s'_n\rangle$ is a zero vector. Acting $O^{D_{\frac{n}{2}}}$ or $O^{D'_{\frac{n}{2}}}$ on other elements $|s''_1,\ldots,s''_n\rangle \in C_n\cdot|s_1,\ldots,s_n\rangle$ will result in a collinear basis vector with a global phase factor of 1 or $-1$.

We now discuss the last situation where $O_j^\theta$ is generated by the diagonal elements in the 2-dimensional irrep. With the irreps as constructed in Eq. 34, the operators become $O_j^\theta = \sum_{i=1}^n A_{jj}^\theta(e_i)e_i$.

We first discuss the operators $O_1^{\theta_j} = \sum_{k=0}^{n-1}\exp(ik\theta_j)C_n^k$. It is trivial to see that the number of elements in the set $\{\exp(ik\theta_j)|0\le k\le n-1, \theta_j=\frac{2\pi j}{n}\}$ must be a factor of $n$ if we notice $C_n^k \mapsto \exp(ik\theta_j)$ is an irrep of $C_n$. Per the orbit-stabilizer theorem[9], the number of elements in $C_n\cdot|s_1,\ldots,s_n\rangle$ is also a factor of $n$. Denoting the number of elements in $C_n\cdot|s_1,\ldots,s_n\rangle$ as $d$, the group actions of $C_n^0, C_n^d, \ldots, C_n^{n-d}$ will keep $|s'_1,\ldots,s'_n\rangle$ unchanged. In $O_1^{\theta_j}\cdot|s'_1,\ldots,s'_n\rangle$, the coefficient of $|s'_1,\ldots,s'_n\rangle$ will be $1+\exp(id\theta_j)+\cdots+\exp(i(n-d)\theta_j)$. This coefficient is nonzero if and only if $d\theta_j$ is a multiple of $2\pi$, or equivalently, if and only if the number of elements in $\{\exp(ik\theta_j)|0\le k\le n-1, \theta_j=\frac{2\pi j}{n}\}$ is a factor of the number of elements in $C_n\cdot|s_1,\ldots,s_n\rangle$. In fact, $1, \exp(id\theta_j), \ldots, \exp(i(n-d)\theta_j)$ are equally spaced complex numbers on the unit circle in the complex plane, and they sum up to zero if $d\theta_j$ is not a multiple of $2\pi$.

The coefficient of another $|s''_1,\ldots,s''_n\rangle \in C_n\cdot|s_1,\ldots,s_n\rangle$ in $O_1^{\theta_j}\cdot|s'_1,\ldots,s'_n\rangle$ is $\exp(ik'\theta_j)+\exp(i(d+k')\theta_j)+\cdots+\exp(i(n-d+k')\theta_j)$, which is $\exp(ik'\theta_j)$ multiplied by the sum in the previous paragraph, where $C_n^{k'}\cdot|s'_1,\ldots,s'_n\rangle = |s''_1,\ldots,s''_n\rangle$. The condition for this coefficient to be zero is the same as that given in the last paragraph. In conclusion, we claim that for any $|s'_1,\ldots,s'_n\rangle \in C_n\cdot|s_1,\ldots,s_n\rangle$, $O_1^{\theta_j}\cdot|s'_1,\ldots,s'_n\rangle$ is a nonzero vector if and only if the number of elements in $\{\exp(ik\theta_j)|0\le k\le n-1, \theta_j=\frac{2\pi j}{n}\}$ is a factor of the number of elements in $C_n\cdot|s_1,\ldots,s_n\rangle$.

The discussion of the operators $O_2^{\theta_j} = \sum_{k=0}^{n-1}\exp(-ik\theta_j)C_n^k$ is similar if we notice that $\exp(-ik\theta_j)$ is the complex conjugate of $\exp(ik\theta_j)$. For any $|s'_1,\ldots,s'_n\rangle \in C_n\cdot|s_1,\ldots,s_n\rangle$, $O_2^{\theta_j}\cdot|s'_1,\ldots,s'_n\rangle$ is a nonzero vector if and only if the number of elements in $\{\exp(-ik\theta_j)|0\le k\le n-1, \theta_j=\frac{2\pi j}{n}\}$ is a factor of the number of elements in $C_n\cdot|s_1,\ldots,s_n\rangle$. When $O_1^{\theta_j}\cdot|s'_1,\ldots,s'_n\rangle$ and $O_2^{\theta_j}\cdot|s'_1,\ldots,s'_n\rangle$ are nonzero, acting $O_1^{\theta_j}$ or $O_2^{\theta_j}$ on another $|s''_1,\ldots,s''_n\rangle \in C_n\cdot|s_1,\ldots,s_n\rangle$ will result in collinear basis vectors with a global phase factor of $\exp(ik'\theta_j)$ or $\exp(-ik'\theta_j)$, respectively, where $C_n^{k'}\cdot|s'_1,\ldots,s'_n\rangle = |s''_1,\ldots,s''_n\rangle$. When $C_n\cdot|s_1,\ldots,s_n\rangle \cap (D_n\backslash C_n)\cdot|s_1,\ldots,s_n\rangle = \varnothing$, the operators $O_1^{\theta_j}$ or $O_2^{\theta_j}$ need to act on two elements in $D_n\cdot|s_1,\ldots,s_n\rangle$ to generate two basis vectors: one element in $C_n\cdot|s_1,\ldots,s_n\rangle$ and the other

in $(D_n \backslash C_n) \cdot |s_1, \ldots, s_n\rangle$.

*Corollary.* Each group algebra element $O_j^\theta$ necessarily acts on zero or one element in the orbit $D_n \cdot |s_1, \ldots, s_n\rangle$ if $C_n \cdot |s_1, \ldots, s_n\rangle = (D_n \backslash C_n) \cdot |s_1, \ldots, s_n\rangle$; or it necessarily acts on zero or two elements in the orbit if $C_n \cdot |s_1, \ldots, s_n\rangle \cap (D_n \backslash C_n) \cdot |s_1, \ldots, s_n\rangle = \varnothing$ to generate the basis vectors. Acting the operator on other elements in the orbit generates a zero vector or a collinear basis vector with no other difference than a global phase factor.

We are now ready to show that these generated basis vectors are orthogonal and complete in the Hilbert space $\mathcal{H}(\mathbb{C}^{2^n})$.

*Orthogonality.* When two different group algebra elements $O_j^\theta$ and $O_{j'}^{\theta'}$ in Eq. 28 act on two elements $|s_1, \ldots, s_n\rangle$ and $|s'_1, \ldots, s'_n\rangle$ in two different orbits, respectively, it is obvious that

$$(\langle s'_1, \ldots, s'_n| O_{j'}^{\theta'})(O_j^\theta |s_1, \ldots, s_n\rangle) = 0 \tag{36}$$

because $O_j^\theta |s_1, \ldots, s_n\rangle$ and $O_{j'}^{\theta'} |s'_1, \ldots, s'_n\rangle$ are in two orthogonal subspaces spanned by the two different orbits.

We discuss the case that the elements $|s_1, \ldots, s_n\rangle$ and $|s'_1, \ldots, s'_n\rangle$ are in the same orbit $D_n \cdot |s''_1, \ldots, s''_n\rangle$. If $O_j^\theta$ and $O_{j'}^{\theta'}$ are both formed by 2-dimensional irreps, obviously, Eq. 36 holds when $|s_1, \ldots, s_n\rangle \in C_n \cdot |s''_1, \ldots, s''_n\rangle$ and $|s'_1, \ldots, s'_n\rangle \in (D_n \backslash C_n) \cdot |s''_1, \ldots, s''_n\rangle$. Otherwise, if $|s_1, \ldots, s_n\rangle$ and $|s'_1, \ldots, s'_n\rangle$ are both in $C_n \cdot |s''_1, \ldots, s''_n\rangle$ or $(D_n \backslash C_n) \cdot |s''_1, \ldots, s''_n\rangle$, without loss of generality, we can assume that $|s_1, \ldots, s_n\rangle = |s'_1, \ldots, s'_n\rangle$ since it results in no other difference than a global phase factor. Letting $O_j^\theta = \sum_{i=1}^n A_{jj}^\theta(e_i) e_i$ and $O_{j'}^{\theta'} = \sum_{i=1}^n A_{j'j'}^{\theta'}(e_i) e_i$, the left-hand side of Eq. 36 becomes $\sum_{i=1}^n (A_{jj}^\theta(e_i) A_{j'j'}^{\theta'}(e_i))$. We can easily see that this is zero with the Schur orthogonality of the irreps of finite groups[6–8].

When at least one of the operators is formed by 1-dimensional irreps, without loss of generality, we can still assume that $|s_1, \ldots, s_n\rangle = |s'_1, \ldots, s'_n\rangle$ in the orbit $D_n \cdot |s''_1, \ldots, s''_n\rangle$ since it results in no other difference than a global phase factor. Letting $O_j^\theta = \sum_{i=1}^{2n} A_{jj}^\theta(e_i) e_i$ and $O_{j'}^{\theta'} = \sum_{i=1}^{2n} A_{j'j'}^{\theta'}(e_i) e_i$, the left-hand side of Eq. 36 becomes $\sum_{i=1}^{2n} (A_{jj}^\theta(e_i) A_{j'j'}^{\theta'}(e_i))$. Again, we directly determine that this is zero with the Schur orthogonality.

*Completeness.* All the elements in all the orbits $D_n \cdot \{|\uparrow\rangle, |\downarrow\rangle\}^{\otimes n}$ together form a complete basis in the Hilbert space $\mathcal{H}(\mathbb{C}^{2^n})$. As such, it is sufficient to show that the operators act on the elements in each orbit the same number of times as the number of elements in that orbit.

The character tables in Tables S3 and S4 list the number of irreps. We first discuss the situation that the orbit $D_n \cdot |s_1, \ldots, s_n\rangle$ has $n$ elements and $C_n \cdot |s_1, \ldots, s_n\rangle = (D_n \backslash C_n) \cdot |s_1, \ldots, s_n\rangle$. If $n$ is odd, the $n-1$ operators generated by the $\frac{n-1}{2}$ 2-dimensional irreps each act on one element in the orbit once. $O^{\mathrm{Id}}$ also acts on the orbit element once. In total, $n$ operators act on the orbit elements.

Otherwise, if $n$ is even, the $n-2$ operators generated by the $\frac{n-2}{2}$ 2-dimensional irreps each act on one element in the orbit once. $O^{\mathrm{Id}}$ also acts on the orbit element once. In addition, one of $O^{D_{\frac{n}{2}}}$ and $O^{D'_{\frac{n}{2}}}$ acts on the orbit element once. In total, $n$ operators act on the orbit elements.

We then discuss the situation that the orbit $D_n \cdot |s_1, \ldots, s_n\rangle$ has $2n$ elements and $C_n \cdot |s_1, \ldots, s_n\rangle \cap (D_n \backslash C_n) \cdot |s_1, \ldots, s_n\rangle = \varnothing$. If $n$ is odd, the $n-1$ operators generated by the $\frac{n-1}{2}$ of 2-dimensional irreps each act on two elements in the orbit once. $O^{\mathrm{Id}}$ and $O^{C_n}$ each acts on one orbit element once. In total, there are $2n$ actions on the orbit elements.

Otherwise, if $n$ is even, the $n-2$ operators generated by the $\frac{n-2}{2}$ of 2-dimensional irreps each act on two elements in the orbit once. $O^{\mathrm{Id}}$ and $O^{C_n}$ each acts on one orbit element once. In addition, both $O^{D_{\frac{n}{2}}}$ and $O^{D'_{\frac{n}{2}}}$ act on one orbit element once. In total, there are $2n$ actions on the orbit elements.

Now we discuss the situation where $D_n \cdot |s_1, \ldots, s_n\rangle$ has fewer than $n$ elements and $C_n \cdot |s_1, \ldots, s_n\rangle = (D_n \backslash C_n) \cdot |s_1, \ldots, s_n\rangle$. Let the number of elements in $D_n \cdot |s_1, \ldots, s_n\rangle$ be $d$, which must be a factor of $n$. In order for an operator $O_1^{\theta_j}$ or $O_2^{\theta_j}$ from a 2-dimensional irrep to act on one element in the orbit and generate a nonzero basis vector, $d$ must be a

multiple of the number of elements in $\{\exp(ik\theta_j)|0 \le k \le n-1, \theta_j = \frac{2\pi j}{n}\}$. This requires $\theta_j$ to be a multiple of $\frac{2\pi}{d}$, or equivalently, $j$ must be a multiple of $\frac{n}{d}$. If $n$ is odd, there are $\frac{d-1}{2}$ of such $j$ satisfying $1 \le j \le \frac{n-1}{2}$; i.e., $\theta_j = \frac{2\pi}{d}, \frac{4\pi}{d}, \ldots, \frac{\pi(d-1)}{d}$; then $d-1$ operators generated by the corresponding $\frac{d-1}{2}$ of 2-dimensional irreps each act on one element in the orbit once. $O^{\mathrm{Id}}$ also acts on the orbit element once. In total, $d$ operators act on the orbit elements.

Otherwise, if $n$ is even, we need to discuss the two situations where $d$ is odd and $d$ is even. When $d$ is odd, there are $\frac{d-1}{2}$ multiples of $\frac{n}{d}$ satisfying $1 \le j \le \frac{n-2}{2}$ (i.e., $\theta_j = \frac{2\pi}{d}, \frac{4\pi}{d}, \ldots, \frac{\pi(d-1)}{d}$). Then $d-1$ operators generated by the corresponding $\frac{d-1}{2}$ of 2-dimensional irreps each act on one element in the orbit once. $O^{\mathrm{Id}}$ also acts on the orbit element once. In total, $d$ operators act on the orbit elements. When $d$ is even, there are $\frac{d-2}{2}$ multiples of $\frac{n}{d}$ satisfying $1 \le j \le \frac{n-2}{2}$ (i.e., $\theta_j = \frac{2\pi}{d}, \frac{4\pi}{d}, \ldots, \frac{\pi(d-2)}{d}$). Then $d-2$ operators generated by the corresponding $\frac{d-2}{2}$ 2-dimensional irreps each act on one element in the orbit once. $O^{\mathrm{Id}}$ and one of $O^{D_{\frac{n}{2}}}$ and $O^{D'_{\frac{n}{2}}}$ also each act on the orbit element once. In total, $d$ operators act on the orbit elements.

Lastly, we discuss the situation where $D_n \cdot |s_1, \ldots, s_n\rangle$ has fewer than $2n$ elements, and $C_n \cdot |s_1, \ldots, s_n\rangle \cap (D_n \backslash C_n) \cdot |s_1, \ldots, s_n\rangle = \varnothing$. This situation is very similar to the situation where $D_n \cdot |s_1, \ldots, s_n\rangle$ has $2n$ elements. In this case, $O^{C_n}$ makes one additional action to $O^{\mathrm{Id}}$, and both $O^{D_{\frac{n}{2}}}$ and $O^{D'_{\frac{n}{2}}}$ make actions if it applies, and each operator generated by the 2-dimensional irreps acts twice if it applies. As a result, the number of actions on the orbit elements is doubled compared with the previous situation.

We have shown that the number of actions on the elements in each orbit is the same as the number of elements in that orbit. These actions generate orthogonal basis vectors, which we have proved. Since all the orbits $D_n \cdot \{|\uparrow\rangle, |\downarrow\rangle\}^{\otimes n}$ together form a complete basis in the Hilbert space $\mathcal{H}(\mathbb{C}^{2^n})$, the basis vectors generated by acting the operators on the orbit elements must also form a complete basis in the Hilbert space $\mathcal{H}(\mathbb{C}^{2^n})$.

*Q.E.D.*

The irreps constructed in Eq. 26 differ from those constructed in Eq. 34; however, they can be transformed into each other with linear unitary transformations. Our conclusion then holds that the basis vectors generated in the procedure of Sec. I D are orthogonal and complete in the Hilbert space $\mathcal{H}(\mathbb{C}^{2^n})$.

It is worth noting that the Schur orthogonality plays an essential role in the proof. Therefore, we claim that the Schur orthogonality and completeness of the irreps of finite groups is the origin of the orthogonality and completeness of the basis vectors generated in the procedure in Sec. I D. We further conjecture that for any subgroup $G$ of $S_n$, a similar procedure of acting the operators defined with the group algebra $\mathcal{R}_G$ on the elements in the orbits $\{G \cdot |s_1, \ldots, s_n\rangle \mid |s_1, \ldots, s_n\rangle \in \{|\uparrow\rangle, |\downarrow\rangle\}^{\otimes n}\}$ will generate an orthogonal and complete basis in the Hilbert space $\mathcal{H}(\mathbb{C}^{2^n})$, and the Schur orthogonality and completeness of the irreps of finite groups will play an essential role in the proof.

### F. Ladder Operators and Selection Rules

In a single qubit system, $\sigma_x$ and $\sigma_y$ form the creation and annihilation operators of the spin; i.e.,

$$\begin{aligned} a_+ &= \frac{1}{2}(\sigma_x + i\sigma_y); \\ a_- &= \frac{1}{2}(\sigma_x - i\sigma_y); \\ a_+|-\rangle &= |+\rangle, a_+|+\rangle = 0; \\ a_-|+\rangle &= |-\rangle, a_-|-\rangle = 0, \end{aligned} \tag{37}$$

where $|+\rangle = |\frac{1}{2}, \frac{1}{2}\rangle$ and $|-\rangle = |\frac{1}{2}, -\frac{1}{2}\rangle$ are in the $|J, M\rangle$ basis. In terms of the $n$-qubit system, the creation and annihilation operator become

$$\begin{aligned}
&A_+ = \frac{1}{2}(H_x + iH_y) = \frac{1}{2}\left(\sum_{i=1}^{n} \sigma_x^{(i)} + i\sum_{i=1}^{n} \sigma_y^{(i)}\right) = \sum_{i=1}^{n} a_+^{(i)};\\
&A_- = \frac{1}{2}(H_x - iH_y) = \frac{1}{2}\left(\sum_{i=1}^{n} \sigma_x^{(i)} - i\sum_{i=1}^{n} \sigma_y^{(i)}\right) = \sum_{i=1}^{n} a_-^{(i)};\\
&A_+|J, M\rangle = c_+(J, M)|J, M+1\rangle \text{ if } M < J; A_+|J, +J\rangle = 0;\\
&A_-|J, M\rangle = c_-(J, M)|J, M-1\rangle \text{ if } M > -J; A_-|J, -J\rangle = 0,
\end{aligned} \tag{38}$$

where $c_+(J, M)$ and $c_-(J, M)$ are coefficients depending on $J, M$. Here $|J, M\rangle$ is the eigenstate of $\tilde{H}_0 = \frac{1}{2}\sum_{i=1}^{n} \sigma_z^{(i)}$, the operator measuring the quantum number $M = \sum_{i=1}^{n} m_s^{(i)}$, in the subspace $\mathcal{H}^J_{[J^{(i)}]}$, i.e.,

$$\tilde{H}_0|J, M\rangle = M|J, M\rangle, |J, M\rangle \in \mathcal{H}^J_{[J^{(i)}]}. \tag{39}$$

When the static field $B_z$ is applied, the eigenenergy of the $|J, M\rangle$ states in the multi-qubit system becomes $B_z M$, i.e.,

$$H_0|J, M\rangle = B_z \cdot \tilde{H}_0|J, M\rangle = B_z M|J, M\rangle. \tag{40}$$

We can then manipulate the energy levels by tuning the amplitude of the static field $B_z$. The creation ($A_+$) and annihilation ($A_-$) operators change the quantum number $M$ by $\pm 1$ but leave $J$ unchanged. Therefore, the evolution of the eigenstates $|J, M\rangle$ is restricted within each subspace $\mathcal{H}^J_{[J^{(i)}]}$ when the Hamiltonians have $S_n$ symmetry as in Eqs. 2 and 4 (this is how the subspaces $\{\mathcal{H}^J_{[J^{(i)}]}\}$ are protected by the $S_n$ symmetry of the system). It should be noted that for each $M \in \{-J, -J+1, \ldots, J-1, J\}$, there is only one basis vector characterized by $M$ (i.e., $|J, M\rangle$) in the subspace $\mathcal{H}^J_{[J^{(i)}]}$. Therefore, the nonzero elements of $A'_+ = A_S^\dagger A_+ A_S$ are at the upper diagonal closest to the main diagonal only, while those of $A'_- = A_S^\dagger A_- A_S$ are at the lower diagonal closest to the main diagonal. Obviously, the value of those nonzero elements are $c_+(J, M)$, and $c_-(J, M)$, respectively. From Eq. 38, it is clear that the nonzero elements of $H'_x = A_S^\dagger H_x A_S$ and $H'_y = A_S^\dagger H_y A_S$ are at the two minor diagonals closest to the main diagonal only, while those of the original $H_x$ and $H_y$ are distributed up to the furthest of the $2^{n-1}$th minor diagonal. When the controlling pulses $B_x(t)$ and $B_y(t)$ are applied, the distribution of the nonzero elements of $H_c$ in Eq. 4 is the same as $H_x$ and $H_y$. Thus, we conclude that the unitary similarity transformation of the Hamiltonians with $A_S$ not only block diagonalizes the Hamiltonians but also reduces the number of nonzero minor diagonals. The simulation of the time-dependent Schrödinger equation in Eq. 1 is accelerated with these two features.

Since the energy levels $\{B_z M | -J \leq M \leq J\}$ of $H_0$ are equally spaced, we assert that the energy spectrum of the multi-qubit system with $S_n$ symmetry resembles that of a simple harmonic oscillator even though there are a finite number of energy levels in each subspace $\mathcal{H}^J_{[J^{(i)}]}$. It should be noted that the control Hamiltonians $H_x$ and $H_y$ can only transition between eigenstates whose $M$ differ by $\pm 1$. Therefore, there is only one resonance frequency of the controlling pulses $B_x(t)$ and $B_y(t)$ that can excite transitions between states. Many desired transitions cannot be realized with a single resonance frequency. To remove the degeneracy in the energy level differences, we introduce coupling terms as in Eq. 3.

The symmetry of the multi-qubit system is reduced to $D_n$ with the introduction of nearest-neighbor coupling terms. Under the action of the $D_n$ elements, the elements in each orbit of $\{|\uparrow\rangle, |\downarrow\rangle\}^{\otimes n}$ have the same numbers of $|\uparrow\rangle$ and $|\downarrow\rangle$ entries, so $M$ is still a good quantum number for the basis vectors in each subspace $\mathcal{H}^\theta_j$. However, more than one basis vector may be characterized by the same $M$ in $\mathcal{H}^\theta_j$. This is because $D_n$ has much

fewer elements than $S_n$. For two elements in $\{|\uparrow\rangle, |\downarrow\rangle\}^{\otimes n}$ to be in the same $D_n$-orbit, they should have the same pattern of spins which is invariant under the $D_n$ actions as well as having the same $M$. Each operator $O_j^\theta$ in Eq. 28 may act on one or two elements in every orbit characterized by the same $M$, and each $M$ may characterize more than one orbit. As such, there may be more than one orthonormal basis vector characterized by the same $M$ in each subspace $\mathcal{H}_j^\theta$. These orthonormal basis vectors of $\mathcal{H}_j^\theta$ are the eigenstates of the coupling Hamiltonian $H_{\text{cpl}} = \sum_{i=1}^{n} \sigma_z^{(i)} \sigma_z^{(i+1)}$, while their eigenvalues are functions of $M$ and the pattern of spins. For 3 qubits and above, the nearest-neighbor coupling terms result in 3 resonance frequencies in the power spectra of the controlling pulses (see Fig. 3f in the main text). Some transitions that are not possible in the $S_n$-symmetry system can now be realized with more resonance frequencies.

Since there may be more than one basis vector characterized by the same $M$ in the subspace $\mathcal{H}_j^\theta$, its dimension is generally larger than that of the subspace $\mathcal{H}_{[J^{(i)}]}^{J}$. Note that the control Hamiltonians $H_x$ and $H_y$ still have $S_n$ symmetry and change $M$ by $\pm 1$. One consequence is that there will be more nonzero upper diagonals in the blocks of $A'_+ = A_D^\dagger A_+ A_D$. This is because any basis vector characterized by $M$ may be transitioned to more than one basis vector characterized by $M \pm 1$. Similarly, there will be more nonzero lower diagonals in the blocks of $A'_- = A_D^\dagger A_- A_D$. Eq. 38 reveals there are more nonzero minor diagonals in $H'_x = A_D^\dagger H_x A_D$ and $H'_y = A_D^\dagger H_y A_D$ compared with those transformed with $A_S$. In other words, more controllability in a multi-qubit system results in an increased subspace dimension and a larger number of nonzero minor diagonals that require more computational resources.

The nonzero elements in $A'_+$ and $A'_-$ determine the selection rules of the multi-qubit system. Even if two eigenstates are in the same subspace, transitions between them can occur only when their $M$ quantum numbers differ by $\pm 1$. When the two states have a larger difference in $M$, the initial state must transition to some intermediate states step by step before it fully transitions to the target state. Under $D_n$ symmetry, in certain circumstances, we are allowed to design a desired "route" (i.e., desired intermediate states) of transitions as long as it is compatible with the selection rules (see Fig. 4c in the main text). Assuming the controlling pulses can be perfectly constructed to be at the required resonance frequencies (i.e., eigenenergy differences between intermediate states in the desired transition), the transition route can be realized by progressing the entire transition with a series of intermediate transitions while each intermediate transition is enabled with a different resonance frequency. The design of the transition routes is possible because the degeneracy of the energy level differences is removed with the $D_n$-symmetry coupling terms. However, when the number of qubits, $n$, is large and the coupling is limited to be between nearest neighbors, some degeneracy of the energy level differences cannot be removed with nearest-neighbor coupling only. Also, some eigenstates with the same $M$ may have the same eigenvalues of $H_{\text{cpl}} = \sum_{i=1}^{n} \sigma_z^{(i)} \sigma_z^{(i+1)}$. Consequently, controlling pulses at some resonance frequency may excite more than one transition simultaneously. The state will then evolve to a linear combination of eigenstates, while the ratio of the coefficients of these eigenstates will be the ratio of the magnitude of corresponding nonzero elements in $A'_+$ and $A'_-$. In this case, none of these eigenstates can be solely transitioned into. To further break the degeneracy of the energy level differences, we introduce the coupling between next nearest neighbors, next next nearest neighbors, and so on.

For the case of nearest-neighbor coupling only, the number of resonance frequencies of the controlling pulses is limited to 3. We can introduce more coupling between qubits that are further from each other, i.e.,

$$
\begin{aligned}
H_0 = B_z \cdot \frac{1}{2} \sum_{i=1}^{n} \sigma_z^{(i)} + c_{\text{cpl}}^{(1)} \cdot \frac{1}{4} \sum_{i=1}^{n} \sigma_z^{(i)} \sigma_z^{(i+1)} + c_{\text{cpl}}^{(2)} \cdot \frac{1}{4} \sum_{i=1}^{n} \sigma_z^{(i)} \sigma_z^{(i+2)} \\
+ \cdots + c_{\text{cpl}}^{(\lfloor \frac{n}{2} \rfloor)} \cdot \frac{1}{4} \sum_{i=1}^{n} \sigma_z^{(i)} \sigma_z^{(i+\lfloor \frac{n}{2} \rfloor)}.
\end{aligned}
\tag{41}
$$

When $n$ is even, we can add coupling terms until the $i$th qubit is coupled to the $(i + \frac{n}{2})$th one because the maximum distance of the indices between two qubits in $\frac{n}{2}$. In contrast, when $n$ is odd, the $i$th qubit can be coupled to the $(i + \frac{n-1}{2})$th one at its extreme. These coupling terms will remove, if not completely, a considerable amount of the degeneracy of the energy levels of the eigenstates characterized by the same $M$. This occurs because the eigenstates with different patterns typically have different eigenvalues. We can then gain more controllability of the multi-qubit system with an increasing number of resonance frequencies. It is worth noting that the coupling strength of each coupling term needs to be carefully tuned, or some of the resonance frequencies will coincide (or be very close to each other), which can be experimentally challenging.

Any transition conserves the angular momentum of the entire physical system. Since the $H_x$ and $H_y$ control Hamiltonians allow transitions between states with $M$ differing by $\pm 1$, the difference of $M$ must be carried by the helicity; i.e., the projection of the spin onto the direction of the momentum of the photon exciting the transition. In this work, we simulate the evolution of the system with a semi-classical model. The controlling pulses are modeled as continuous electromagnetic waves during a finite time span. As such, the helicity of photons is manifested by its classical counterpart, the polarization of electromagnetic waves. Only one handedness of the circularly polarized light, either left-handed or right-handed, is able to excite a specific transition. If the sign of the static Hamiltonian $H_0$ is changed (i.e., $H_0 \mapsto -H_0$), the other handedness will be selected. The controlling pulses modeled in only one direction, either along the $x$- or $y$-axis, can be linearly polarized only. To simulate circularly polarized light, we manipulate the multi-qubit system with both $B_x(t)$ and $B_y(t)$.

## II. SUPPLEMENTARY FIGURES

### A. Supplementary Sparsity Plots for Hamiltonians

We provide sparsity plots for Hamiltonians of the 3-, 4-, 5-, and 7-qubit systems. These figures supplement Fig. 2 in the main text. It is worth noting that $A_S^\dagger H_{z,\mathrm{cpl}} A_S$ in the 3-qubit system is block diagonalized because $S_3 = D_3$ and consequently, $A_{S_3} = A_{D_3}$.

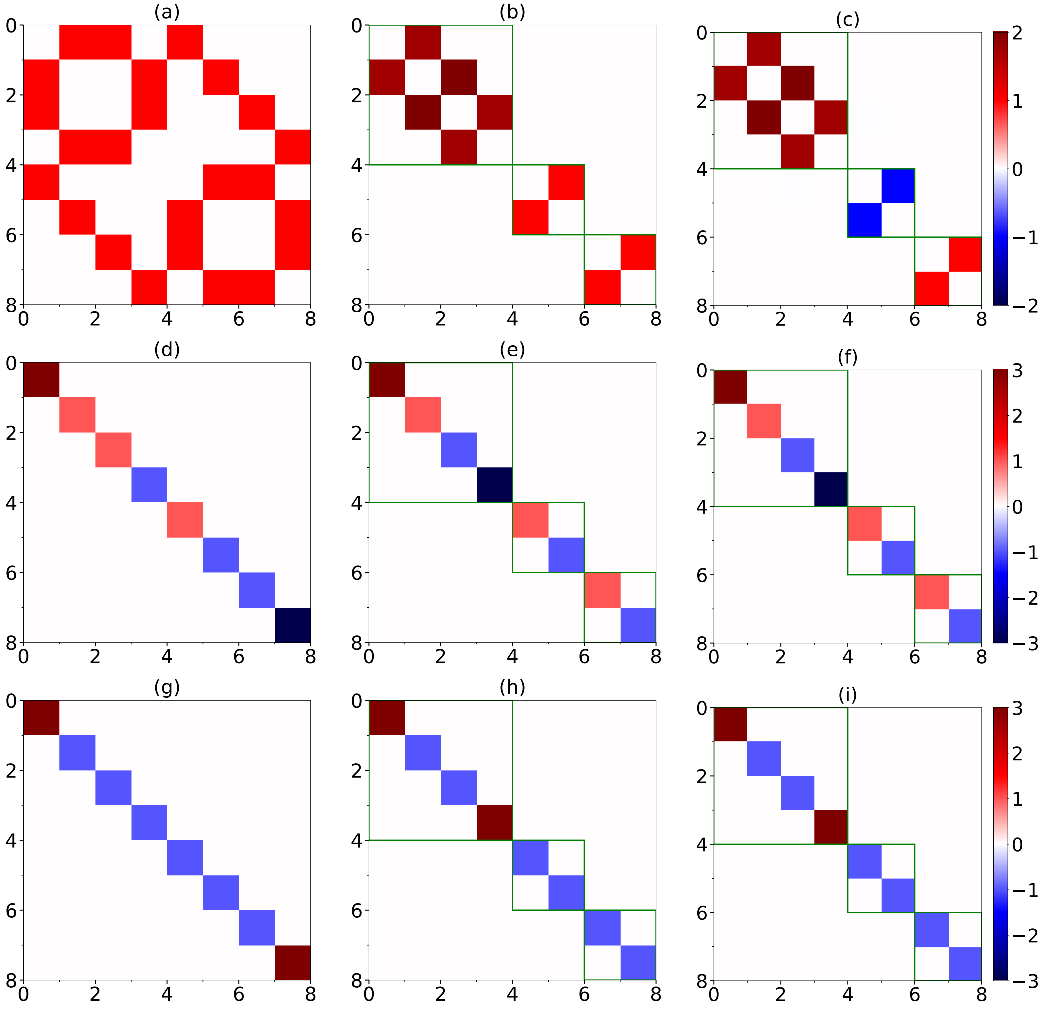


Figure S2: **Sparsity plots for Hamiltonians of a 3-qubit system.** (a) $H_x$; (b) $A_S^\dagger H_x A_S$; (c) $A_D^\dagger H_x A_D$; (d) $H_z$; (e) $A_S^\dagger H_z A_S$; (f) $A_D^\dagger H_z A_D$; (g) $H_{z,\mathrm{cpl}}$; (h) $A_S^\dagger H_{z,\mathrm{cpl}} A_S$; and (i) $A_D^\dagger H_{z,\mathrm{cpl}} A_D$. The $x$- and $y$-axes denote the column and row indices of the matrix elements, respectively. The color bars indicate the value of the matrix elements. Each block for the matrices in panels (b), (c), (e), (f), (h), and (i) is enclosed by a green-colored square box.

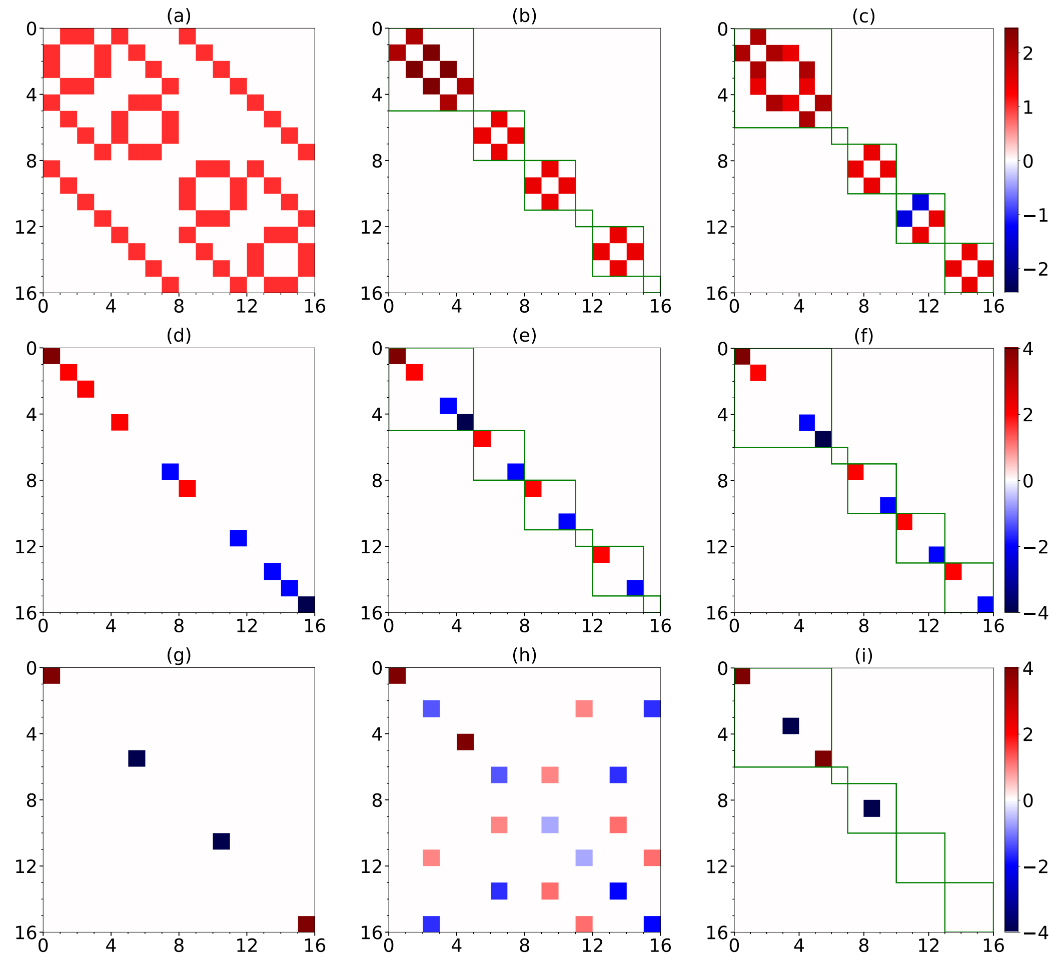


Figure S3: **Sparsity plots for Hamiltonians of a 4-qubit system.** (a) $H_x$; (b) $A_S^\dagger H_x A_S$; (c) $A_D^\dagger H_x A_D$; (d) $H_z$; (e) $A_S^\dagger H_z A_S$; (f) $A_D^\dagger H_z A_D$; (g) $H_{z,\mathrm{cpl}}$; (h) $A_S^\dagger H_{z,\mathrm{cpl}} A_S$; and (i) $A_D^\dagger H_{z,\mathrm{cpl}} A_D$. The $x$- and $y$-axes denote the column and row indices of the matrix elements, respectively. The color bars indicate the value of the matrix elements. Each block for the matrices in panels (b), (c), (e), (f), and (i) is enclosed by a green-colored square box.

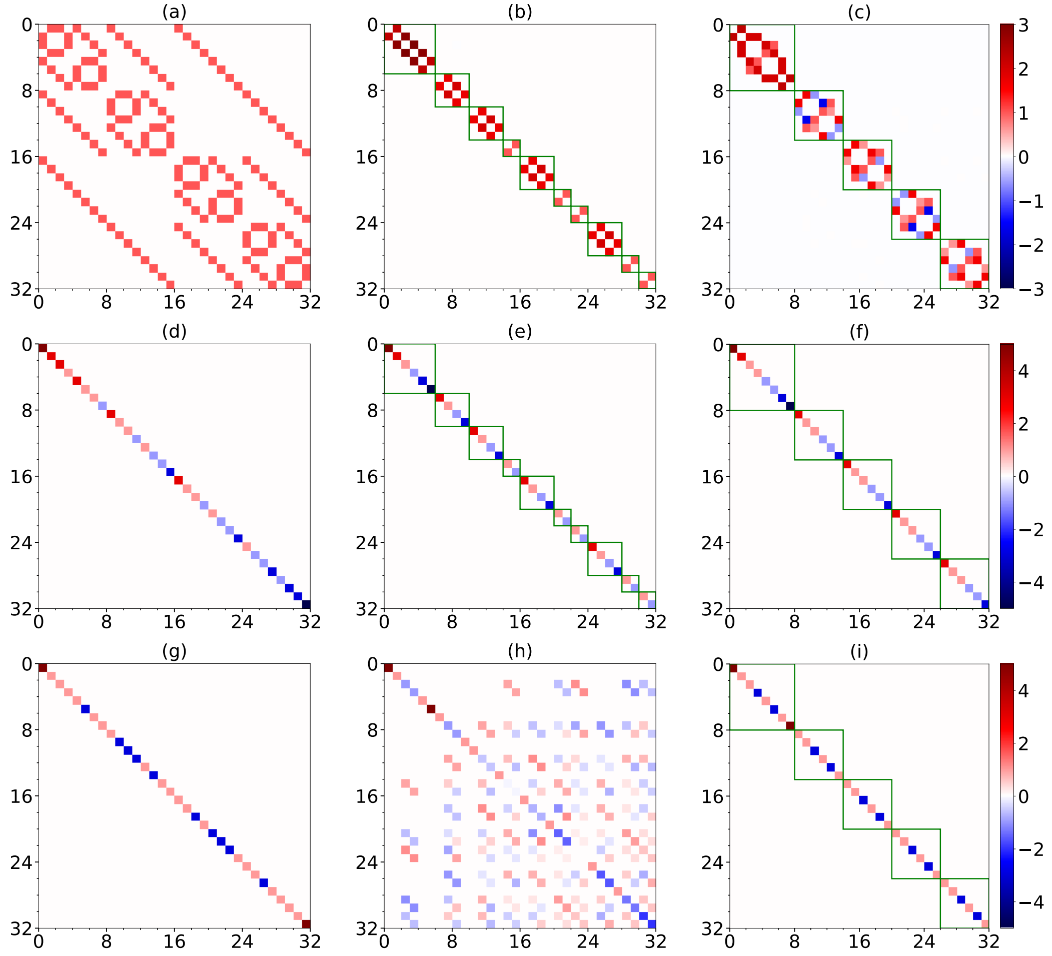


Figure S4: **Sparsity plots for Hamiltonians of a 5-qubit system.** (a) $H_x$; (b) $A_S^\dagger H_x A_S$; (c) $A_D^\dagger H_x A_D$; (d) $H_z$; (e) $A_S^\dagger H_z A_S$; (f) $A_D^\dagger H_z A_D$; (g) $H_{z,\mathrm{cpl}}$; (h) $A_S^\dagger H_{z,\mathrm{cpl}} A_S$; and (i) $A_D^\dagger H_{z,\mathrm{cpl}} A_D$. The $x$- and $y$-axes denote the column and row indices of the matrix elements, respectively. The color bars indicate the value of the matrix elements. Each block for the matrices in panels (b), (c), (e), (f), and (i) is enclosed by a green-colored square box.

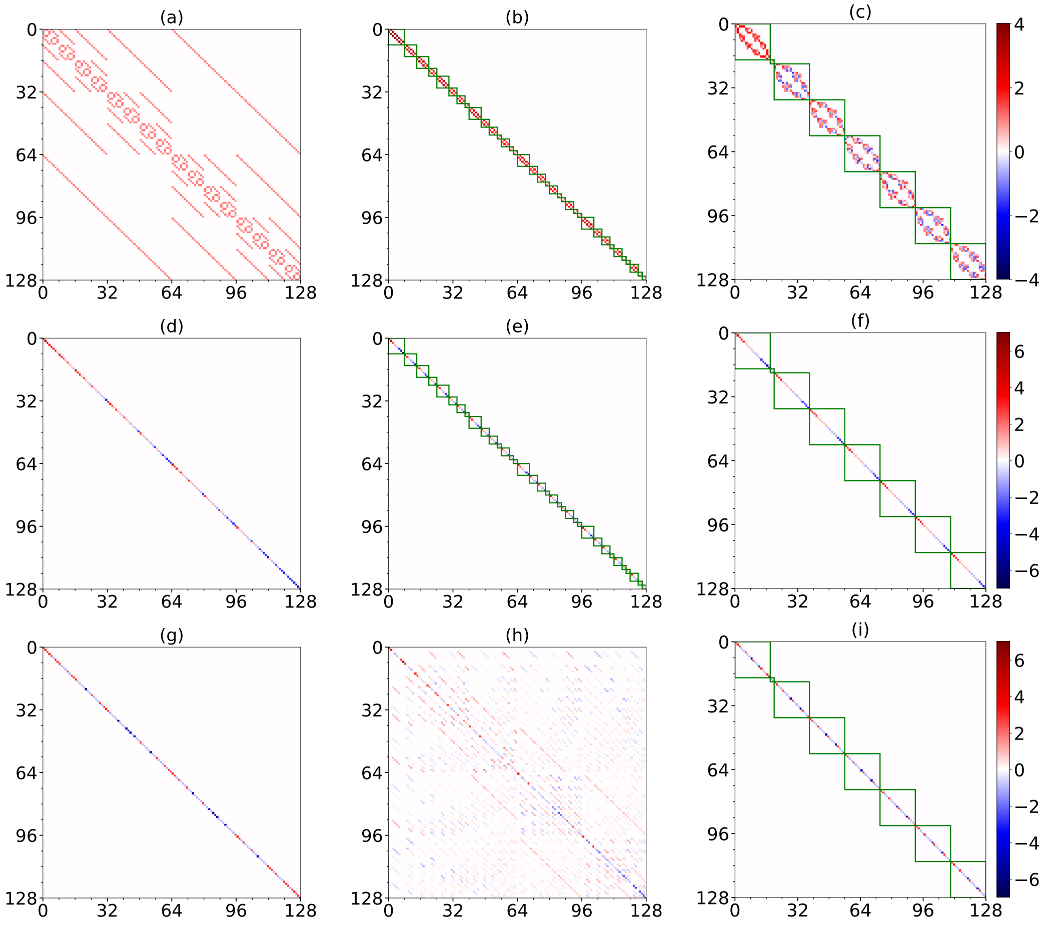


Figure S5: **Sparsity plots for Hamiltonians of a 7-qubit system.** (a) $H_x$; (b) $A_S^\dagger H_x A_S$; (c) $A_D^\dagger H_x A_D$; (d) $H_z$; (e) $A_S^\dagger H_z A_S$; (f) $A_D^\dagger H_z A_D$; (g) $H_{z,\mathrm{cpl}}$; (h) $A_S^\dagger H_{z,\mathrm{cpl}} A_S$; and (i) $A_D^\dagger H_{z,\mathrm{cpl}} A_D$. The $x$- and $y$-axes denote the column and row indices of the matrix elements, respectively. The color bars indicate the value of the matrix elements. Each block for the matrices in panels (b), (c), (e), (f), and (i) is enclosed by a green-colored square box.

## B. Supplementary Plots of Optimal Control Pulses

We provide plots of optimal control pulses generated by the original and symmetry-based methods for the 6-, 7-, and 8-qubit systems. These figures supplement Fig. 3c and d in the main text.

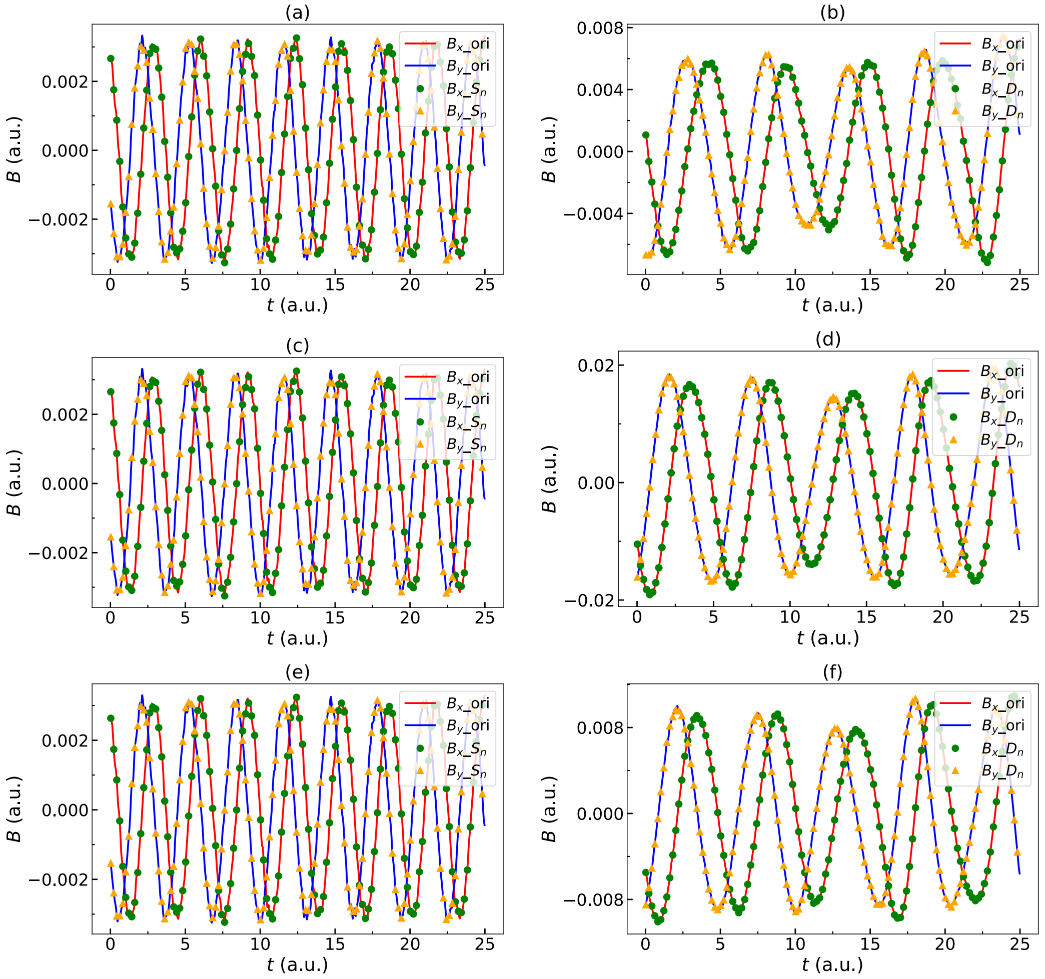


Figure S6: **Comparison of optimal control pulses between the original and symmetry-based methods.** Optimized $B_x(t)$ and $B_y(t)$ pulses for non-coupled and nearest-neighbor-coupled systems with (a), (b) 6 qubits; (c), (d) 7 qubits; and (e), (f) 8 qubits.

### C. Supplementary Plots of the Power Spectra and Convergence

We provide plots of the power spectra of the optimized pulses and probability vs. iteration for the 5- and 6-qubit system, with nearest-neighbor coupling and full coupling, respectively. These figures supplement Fig. 4d and e in the main text. It should be noted that in Fig. S7a, the frequencies of the three resonance peaks of the nearest-neighbor-coupled 5-qubit system (plotted in red), i.e., $1.2, 2, 2.8$ a.u., coincide with the frequencies of the resonance peaks of the fully coupled 5-qubit system (plotted in blue).

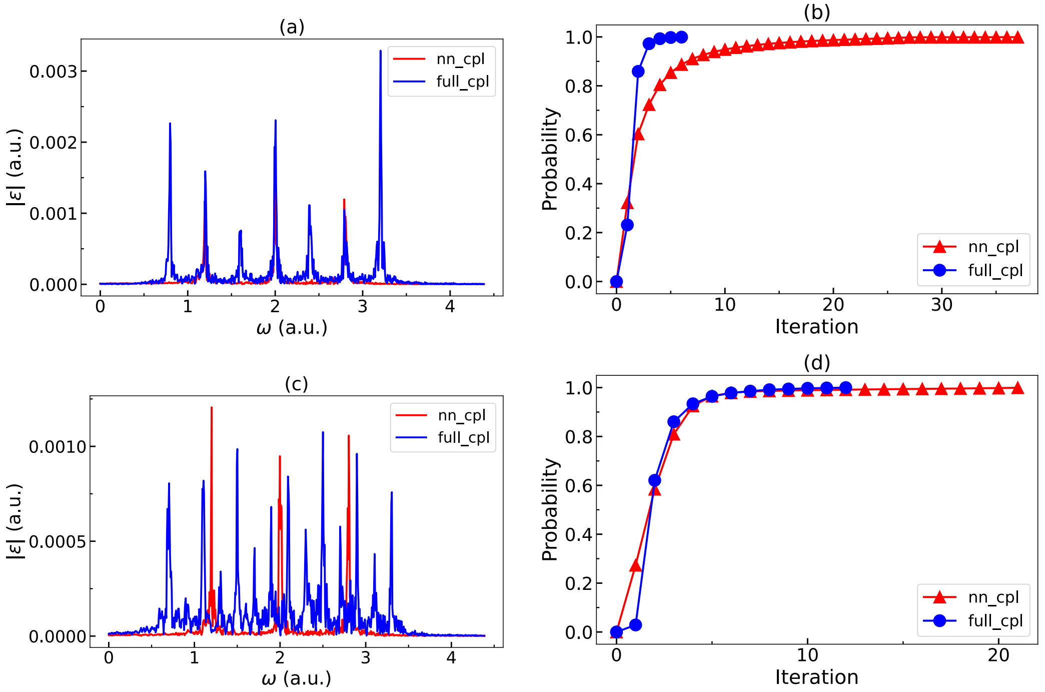


Figure S7: **Power spectra and convergence of the system with nearest-neighbor and full coupling.** Power spectra of the optimized pulses when the (a) 5-; (c) and 6-qubit system has nearest-neighbor coupling and full coupling, respectively. Comparison of probability vs. iteration when the (b) 5- and (d) 6-qubit system has nearest-neighbor and full coupling.

## REFERENCES

[1] Dawei Lu, Keren Li, Jun Li, Hemant Katiyar, Annie Jihyun Park, Guanru Feng, Tao Xin, Hang Li, Guilu Long, Aharon Brodutch, Jonathan Baugh, Bei Zeng, and Raymond Laflamme. Enhancing quantum control by bootstrapping a quantum processor of 12 qubits. *npj Quantum Information*, 3(1):45, Oct 2017.

[2] Peter Štelmachovič and Vladimír Bužek. Quantum-information approach to the Ising model: Entanglement in chains of qubits. *Physical Review A*, 70(3):032313, 2004.

[3] Chao Song, Kai Xu, Hekang Li, Yu-Ran Zhang, Xu Zhang, Wuxin Liu, Qiujiang Guo, Zhen Wang, Wenhui Ren, Jie Hao, et al. Generation of multicomponent atomic schrödinger cat states of up to 20 qubits. *Science*, 365(6453):574–577, 2019.

[4] Navin Khaneja, Timo Reiss, Cindie Kehlet, Thomas Schulte-Herbrüggen, and Steffen J Glaser. Optimal control of coupled spin dynamics: Design of NMR pulse sequences by gradient ascent algorithms. *Journal of Magnetic Resonance*, 172(2):296–305, 2005.

[5] Akber Raza, Chengkuan Hong, Xian Wang, Anshuman Kumar, Christian R. Shelton, and Bryan M. Wong. NIC-CAGE: An open-source software package for predicting optimal control fields in photo-excited chemical systems. *Computer Physics Communications*, 258:107541, 2021.

[6] Zhong-Qi Ma. In *Group Theory for Physicists (Second Edition)*, pages 49–276. World Scientific Publishing Co. Pte. Ltd., 2007.

[7] Qi-Zhi Han and Hong-Zhou Sun. In *Group Theory*, pages 28–184. Peking University Press, 1987.

[8] Xin-Zheng Li. In *Group Theory and its Application to Condensed Matter Physics*, pages 41–199, 260–328. Peking University Press, 2019.

[9] Minking Eie and Shou-Te Chang. In *A Course on Abstract Algebra*, pages 144–151. World Scientific Publishing Co. Pte. Ltd., 2010.
